# Supplementary material for: On conformal higher spin wave operators
Source: arXiv:1404.7452 ancillary file (2014-07-08)
Supplement: Supplementary file 1 [file conformal_spin_3_in_4d.nb.pdf]

# Conformal spin 3 on arbitrary 4d backgrounds

## Existence and obstruction to factorization

Teake Nutma and Massimo Taronna

Max Planck Institute for Gravitational Physics (Albert Einstein Institute)  
(Albert Einstein Institut)  
Am Mühlenberg 1,  
14476 Golm, Germany

{teake.nutma, massimo.taronna}@aei.mpg.de

In[72]:= **DateString[]**

Out[72]:= Tue 29 Apr 2014 09:15:07

---

## Introduction

### Summary

In this notebook we conjecture the existence of a unique quadratic action for a traceless symmetric spin-3 field  $\varphi_{abc}$ , minimally coupled to Weyl gravity,

$$S = \int d^4x \sqrt{-g} \left( W^2 + \frac{1}{2} \varphi_{abc} O^{abcdef} \varphi_{def} \right), \quad (1)$$

(latin indices are curved) which is invariant under the gauge transformations

$$\begin{aligned} \delta_\xi \varphi_{abc} &= P \nabla_{(a} \xi_{bc)}, \\ \delta_\xi g_{ab} &= (\varphi \nabla \nabla \nabla \xi)_{ab} + \dots, \end{aligned} \quad (2)$$

and invariant under the Weyl rescalings

$$\begin{aligned} \varphi_{abc} &\rightarrow e^{4\Omega} \varphi_{abc}, \\ g_{ab} &\rightarrow e^{2\Omega} g_{ab}. \end{aligned} \quad (3)$$

The existence is a conjecture, because we work only linearly in the Riemann tensor. That is, terms containing  $R^2$  or higher powers are neglected.

The operator  $O_{abc}^{def}$  has six derivatives. It does not factorize into three operators with two derivatives on general backgrounds. We show that the obstruction for factorization is the first derivative of the Weyl tensor.

### Final equations of motion

We now present the final result for the spin 3 equations of motion that follow from the action  $S$  (1). First, on AdS backgrounds, they read

In[391]:= **spin3equationsofmotion /. SymmetricSpaceRules[CD, Δ] // CollectTensors**

$$\begin{aligned} \text{Out[391]} = & -\frac{21}{5} \Delta \text{Ttf}^{abc} (\nabla_{(bcde)} \varphi_a^{de}) + \frac{42}{5} \Delta \text{Ttf}^{abc} (\nabla_{(cd^e e)} \varphi_{ab}^d) - \\ & \frac{7}{2} \Delta \text{Ttf}^{abc} (\nabla_{(d^e e)} \varphi_{abc}) - \frac{2}{5} \text{Ttf}^{abc} (\nabla_{(abcdef)} \varphi^{def}) + \\ & \frac{12}{5} \text{Ttf}^{abc} (\nabla_{(bcde f)} \varphi_a^{de}) - 3 \text{Ttf}^{abc} (\nabla_{(cd^e e f)} \varphi_{ab}^d) + \text{Ttf}^{abc} (\nabla_{(d^e e f)} \varphi_{abc}) = 0 \end{aligned}$$

Here  $\text{Ttf}_{abc}$  is an auxiliary traceless tensor that simply contracts the free indices.

On Ricci-flat backgrounds, they read

In[392]:= **spin3equationsofmotion /. RiemannCD[\_\_\_\_, a\_, \_\_\_\_, b\_, \_\_\_\_] ;; PairQ[a, b] → 0 /.  
CD[\_\_\_\_, a\_, \_\_\_\_] @RiemannCD[\_\_\_\_, b\_, \_\_\_\_] ;; PairQ[a, b] → 0**

$$\begin{aligned} \text{Out[392]} = & \frac{49}{25} \text{Ttf}^{abc} (\nabla_{(bc)} R[\nabla]_{aefg}) (\nabla_{(d}^g \varphi^{def}) - \\ & 7 \text{Ttf}^{abc} (\nabla_{(cf)} R[\nabla]_{aebg}) (\nabla_{(d}^g \varphi^{def}) - \frac{49}{25} \text{Ttf}^{abc} (\nabla_{(cg)} R[\nabla]_{aebf}) (\nabla_{(d}^g \varphi^{def}) - \\ & \frac{84}{25} \text{Ttf}^{abc} (\nabla_{(a}^g \varphi^{def}) (\nabla_{(ef)} R[\nabla]_{bdcg}) - \frac{259}{25} \text{Ttf}^{abc} (\nabla_{(a}^g \varphi^{def}) (\nabla_{(fg)} R[\nabla]_{bdce}) + \\ & \frac{7}{10} \text{Ttf}^{abc} (\nabla_{(ce)} R[\nabla]_{bfdg}) (\nabla_{(fg)} \varphi_a^{de}) - \frac{161}{50} \text{Ttf}^{abc} (\nabla_{(de)} R[\nabla]_{bfcg}) (\nabla_{(fg)} \varphi_a^{de}) + \\ & \frac{721}{50} \text{Ttf}^{abc} (\nabla_{(eg)} R[\nabla]_{bdcf}) (\nabla_{(fg)} \varphi_a^{de}) + \\ & \frac{182}{25} \text{Ttf}^{abc} (\nabla_{(fg)} R[\nabla]_{bdce}) (\nabla_{(fg)} \varphi_a^{de}) - \frac{21}{10} \text{Ttf}^{abc} (\nabla_{(cf)} R[\nabla]_{adbe}) (\nabla_{(g}^g \varphi^{def}) - \\ & \frac{21}{5} \text{Ttf}^{abc} (\nabla_{(ad)} \varphi^{def}) (\nabla_{(g}^g R[\nabla]_{becf}) + \frac{252}{25} \text{Ttf}^{abc} (\nabla_{(d}^f \varphi_a^{de}) (\nabla_{(g}^g R[\nabla]_{becf}) - \\ & \frac{343}{50} \text{Ttf}^{abc} (\nabla_{(b}^f \varphi_a^{de}) (\nabla_{(g}^g R[\nabla]_{cdef}) + \frac{35}{2} \text{Ttf}^{abc} (\nabla_{(ef)} \varphi_{ab}^d) (\nabla_{(g}^g R[\nabla]_{cedf}) + \\ & \frac{7}{5} \text{Ttf}^{abc} (\nabla^g R[\nabla]_a^{def}) (\nabla_{(bcf)} \varphi_{deg}) - \frac{7}{50} \text{Ttf}^{abc} (\nabla^g \varphi^{def}) (\nabla_{(bcf)} R[\nabla]_{adeg}) - \\ & \frac{441}{50} \text{Ttf}^{abc} (\nabla^g R[\nabla]_a^{def}) (\nabla_{(cdf)} \varphi_{beg}) - \frac{21}{10} \text{Ttf}^{abc} (\nabla^g \varphi^{def}) (\nabla_{(cef)} R[\nabla]_{adbg}) + \\ & \frac{161}{50} \text{Ttf}^{abc} (\nabla_a R[\nabla]^{defg}) (\nabla_{(ceg)} \varphi_{bdf}) - \frac{49}{5} \text{Ttf}^{abc} (\nabla^f R[\nabla]_a^{de}) (\nabla_{(ceg)} \varphi_{df}^g) - \\ & \frac{399}{50} \text{Ttf}^{abc} (\nabla^g R[\nabla]_a^{def}) (\nabla_{(cfg)} \varphi_{bde}) + 7 \text{Ttf}^{abc} (\nabla_b R[\nabla]_a^{def}) (\nabla_{(cfg)} \varphi_{de}^g) - \\ & \frac{42}{5} \text{Ttf}^{abc} (\nabla^f R[\nabla]_a^{de}) (\nabla_{(cfg)} \varphi_{de}^g) - \frac{203}{50} \text{Ttf}^{abc} (\nabla^g \varphi^{def}) (\nabla_{(cfg)} R[\nabla]_{adbe}) - \\ & \frac{42}{5} \text{Ttf}^{abc} (\nabla^f R[\nabla]_a^{de}) (\nabla_{(c}^g \varphi_{def}) - \frac{42}{25} \text{Ttf}^{abc} (\nabla_d \varphi^{def}) (\nabla_{(c}^g R[\nabla]_{aebf}) - \\ & \frac{98}{25} \text{Ttf}^{abc} (\nabla^f \varphi_a^{de}) (\nabla_{(c}^g R[\nabla]_{bdef}) - \frac{161}{50} \text{Ttf}^{abc} (\nabla^f R[\nabla]_a^{de}) (\nabla_{(deg)} \varphi_{cf}^g) + \\ & \frac{98}{5} \text{Ttf}^{abc} (\nabla^g R[\nabla]_a^{def}) (\nabla_{(dfg)} \varphi_{bce}) - \frac{399}{50} \text{Ttf}^{abc} (\nabla_b R[\nabla]_a^{def}) (\nabla_{(dfg)} \varphi_{ce}^g) + \\ & \frac{721}{50} \text{Ttf}^{abc} (\nabla^f R[\nabla]_a^{de}) (\nabla_{(efg)} \varphi_{cd}^g) - 7 \text{Ttf}^{abc} (\nabla_c R[\nabla]_a^{de}) (\nabla_{(efg)} \varphi_d^{fg}) + \\ & \frac{56}{5} \text{Ttf}^{abc} (\nabla^f R[\nabla]_a^{de}) (\nabla_{(e}^g \varphi_{cdf}) + \frac{154}{25} \text{Ttf}^{abc} (\nabla^f \varphi_a^{de}) (\nabla_{(e}^g R[\nabla]_{bdcf}) + \end{aligned}$$

$$\begin{aligned}
& \frac{42}{5} \text{Ttf}^{abc} \left( \nabla^f R[\nabla]_a{}^d{}_b{}^e \right) \left( \nabla_{(f}{}^g{}_{g)} \varphi_{cde} \right) - \frac{112}{25} \text{Ttf}^{abc} \left( \nabla_a \varphi^{def} \right) \left( \nabla_{(f}{}^g{}_{g)} R[\nabla]_{bdce} \right) + \\
& \frac{77}{25} \text{Ttf}^{abc} \left( \nabla^f \varphi_a{}^{de} \right) \left( \nabla_{(f}{}^g{}_{g)} R[\nabla]_{bdce} \right) + \frac{42}{5} R[\nabla]_a{}^{def} \text{Ttf}^{abc} \left( \nabla_{(bcfg)} \varphi_{de}{}^g \right) - \\
& \frac{84}{5} R[\nabla]_a{}^{def} \text{Ttf}^{abc} \left( \nabla_{(cdfg)} \varphi_{be}{}^g \right) - \frac{42}{5} R[\nabla]_a{}^d{}_b{}^e \text{Ttf}^{abc} \left( \nabla_{(cefg)} \varphi_d{}^{fg} \right) - \\
& \frac{56}{5} R[\nabla]_a{}^{def} \text{Ttf}^{abc} \left( \nabla_{(cfg)} \varphi_{bde} \right) - \frac{42}{5} R[\nabla]_a{}^d{}_b{}^e \text{Ttf}^{abc} \left( \nabla_{(cfg)} \varphi_{de}{}^f \right) - \\
& \frac{36}{5} \varphi^{abc} \text{Ttf}^{def} \left( \nabla_{(cfg)} R[\nabla]_{adbe} \right) + \frac{98}{5} R[\nabla]_a{}^{def} \text{Ttf}^{abc} \left( \nabla_{(dfg)} \varphi_{bce} \right) + \\
& \frac{56}{5} R[\nabla]_a{}^d{}_b{}^e \text{Ttf}^{abc} \left( \nabla_{(efg)} \varphi_{cd}{}^f \right) + \frac{21}{5} R[\nabla]_a{}^d{}_b{}^e \text{Ttf}^{abc} \left( \nabla_{(fg)} \varphi_{cde} \right) - \\
& \frac{2}{5} \text{Ttf}^{abc} \left( \nabla_{(abcdef)} \varphi^{def} \right) + \frac{12}{5} \text{Ttf}^{abc} \left( \nabla_{(bcde)} \varphi_a{}^{de} \right) - \\
& 3 \text{Ttf}^{abc} \left( \nabla_{(cde)} \varphi_{ab}{}^d \right) + \text{Ttf}^{abc} \left( \nabla_{(de)} \varphi_{abc} \right) = 0
\end{aligned}$$

Lastly, the full equations of motion read:

In[383]:= **spin3equationsofmotion**

$$\begin{aligned}
\text{Out[383]} = & -\frac{21}{10} \text{Ttf}^{abc} \left( \nabla_{(cg)} R[\nabla]_{afb}{}^g \right) \left( \nabla_{(de)} \varphi^{def} \right) + \frac{49}{25} \text{Ttf}^{abc} \left( \nabla_{(bc)} R[\nabla]_{aefg} \right) \left( \nabla_d{}^g \varphi^{def} \right) - \\
& 7 \text{Ttf}^{abc} \left( \nabla_{(cf)} R[\nabla]_{aebg} \right) \left( \nabla_d{}^g \varphi^{def} \right) - \frac{49}{25} \text{Ttf}^{abc} \left( \nabla_{(cg)} R[\nabla]_{aebf} \right) \left( \nabla_d{}^g \varphi^{def} \right) - \\
& \frac{84}{25} \text{Ttf}^{abc} \left( \nabla_{(a)}{}^g \varphi^{def} \right) \left( \nabla_{(ef)} R[\nabla]_{bdcg} \right) - \frac{42}{5} \text{Ttf}^{abc} \left( \nabla_{(ad)} \varphi^{def} \right) \left( \nabla_{(ef)} R[\nabla]_{b}{}^g{}_{cg} \right) + \\
& \frac{77}{25} \text{Ttf}^{abc} \left( \nabla_{(d)}{}^f \varphi_a{}^{de} \right) \left( \nabla_{(ef)} R[\nabla]_{b}{}^g{}_{cg} \right) - \frac{21}{5} \text{Ttf}^{abc} \left( \nabla_{(ab)} \varphi^{def} \right) \left( \nabla_{(ef)} R[\nabla]_{c}{}^g{}_{dg} \right) + \\
& \frac{217}{25} \text{Ttf}^{abc} \left( \nabla_{(b)}{}^f \varphi_a{}^{de} \right) \left( \nabla_{(ef)} R[\nabla]_{c}{}^g{}_{dg} \right) - \frac{21}{25} \text{Ttf}^{abc} \left( \nabla_{(d)}{}^f \varphi_a{}^{de} \right) \left( \nabla_{(eg)} R[\nabla]_{bfc}{}^g \right) + \\
& \frac{959}{50} \text{Ttf}^{abc} \left( \nabla_{(b)}{}^f \varphi_a{}^{de} \right) \left( \nabla_{(eg)} R[\nabla]_{cfd}{}^g \right) - \frac{28}{5} \text{Ttf}^{abc} \left( \nabla_{(bd)} \varphi_a{}^{de} \right) \left( \nabla_{(eg)} R[\nabla]_{c}{}^f{}_{fg} \right) - \\
& \frac{1001}{50} \text{Ttf}^{abc} \left( \nabla_{(b)}{}^f \varphi_a{}^{de} \right) \left( \nabla_{(eg)} R[\nabla]_{c}{}^g{}_{df} \right) + \\
& \frac{14}{5} \text{Ttf}^{abc} \left( \nabla_{(bc)} \varphi_a{}^{de} \right) \left( \nabla_{(eg)} R[\nabla]_{d}{}^f{}_{fg} \right) - \frac{7}{5} \text{Ttf}^{abc} \left( \nabla_{(c)}{}^e \varphi_{ab}{}^d \right) \left( \nabla_{(eg)} R[\nabla]_{d}{}^f{}_{fg} \right) + \\
& \frac{21}{5} \text{Ttf}^{abc} \left( \nabla_{(df)} R[\nabla]_{c}{}^g{}_{eg} \right) \left( \nabla^{(ef)} \varphi_{ab}{}^d \right) - \frac{7}{5} \text{Ttf}^{abc} \left( \nabla_{(dg)} R[\nabla]_{cef}{}^g \right) \left( \nabla^{(ef)} \varphi_{ab}{}^d \right) - \\
& \frac{77}{10} \text{Ttf}^{abc} \left( \nabla_{(ef)} R[\nabla]_{c}{}^g{}_{dg} \right) \left( \nabla^{(ef)} \varphi_{ab}{}^d \right) - \frac{259}{25} \text{Ttf}^{abc} \left( \nabla_{(a)}{}^g \varphi^{def} \right) \left( \nabla_{(fg)} R[\nabla]_{bdce} \right) - \\
& 21 \text{Ttf}^{abc} \left( \nabla_{(ad)} \varphi^{def} \right) \left( \nabla_{(fg)} R[\nabla]_{bec}{}^g \right) + \frac{364}{25} \text{Ttf}^{abc} \left( \nabla_{(d)}{}^f \varphi_a{}^{de} \right) \left( \nabla_{(fg)} R[\nabla]_{bec}{}^g \right) - \\
& \frac{21}{2} \text{Ttf}^{abc} \left( \nabla_{(ab)} \varphi^{def} \right) \left( \nabla_{(fg)} R[\nabla]_{cde}{}^g \right) + \frac{119}{50} \text{Ttf}^{abc} \left( \nabla_{(b)}{}^f \varphi_a{}^{de} \right) \left( \nabla_{(fg)} R[\nabla]_{cde}{}^g \right) - \\
& \frac{77}{10} \text{Ttf}^{abc} \left( \nabla^{(ef)} \varphi_{ab}{}^d \right) \left( \nabla_{(fg)} R[\nabla]_{ced}{}^g \right) + \frac{231}{10} \text{Ttf}^{abc} \left( \nabla^{(ef)} \varphi_{ab}{}^d \right) \left( \nabla_{(fg)} R[\nabla]_{c}{}^g{}_{de} \right) - \\
& \frac{14}{5} \text{Ttf}^{abc} \left( \nabla_{(bc)} \varphi_a{}^{de} \right) \left( \nabla_{(fg)} R[\nabla]_{d}{}^f{}_{eg} \right) + \frac{7}{5} \text{Ttf}^{abc} \left( \nabla_{(c)}{}^e \varphi_{ab}{}^d \right) \left( \nabla_{(fg)} R[\nabla]_{d}{}^f{}_{eg} \right) - \\
& \frac{7}{50} \text{Ttf}^{abc} \left( \nabla_{(ce)} R[\nabla]_{b}{}^g{}_{dg} \right) \left( \nabla_{(f)}{}^f \varphi_a{}^{de} \right) + \frac{217}{50} \text{Ttf}^{abc} \left( \nabla_{(de)} R[\nabla]_{b}{}^g{}_{cg} \right) \left( \nabla_{(f)}{}^f \varphi_a{}^{de} \right) +
\end{aligned}$$

$$\begin{aligned}
& \frac{623}{50} \text{Ttf}^{abc} \left( \nabla_{(eg)} R[\nabla]_{bdc}{}^g \right) \left( \nabla^{(f)}{}_{(f)} \varphi_a{}^{de} \right) + \\
& \frac{7}{10} \text{Ttf}^{abc} \left( \nabla_{(ce)} R[\nabla]_{bfdg} \right) \left( \nabla^{(fg)} \varphi_a{}^{de} \right) - \frac{161}{50} \text{Ttf}^{abc} \left( \nabla_{(de)} R[\nabla]_{bfcg} \right) \left( \nabla^{(fg)} \varphi_a{}^{de} \right) + \\
& \frac{721}{50} \text{Ttf}^{abc} \left( \nabla_{(eg)} R[\nabla]_{bdcf} \right) \left( \nabla^{(fg)} \varphi_a{}^{de} \right) + \\
& \frac{182}{25} \text{Ttf}^{abc} \left( \nabla_{(fg)} R[\nabla]_{bdce} \right) \left( \nabla^{(fg)} \varphi_a{}^{de} \right) - \frac{21}{10} \text{Ttf}^{abc} \left( \nabla_{(cf)} R[\nabla]_{adbe} \right) \left( \nabla^{(g)}{}_{(g)} \varphi^{def} \right) - \\
& \frac{21}{5} \text{Ttf}^{abc} \left( \nabla_{(ad)} \varphi^{def} \right) \left( \nabla^{(g)}{}_{(g)} R[\nabla]_{becf} \right) + \frac{252}{25} \text{Ttf}^{abc} \left( \nabla_{(d)}{}^{(f)} \varphi_a{}^{de} \right) \left( \nabla^{(g)}{}_{(g)} R[\nabla]_{becf} \right) - \\
& \frac{21}{5} \text{Ttf}^{abc} \left( \nabla_{(de)} \varphi_a{}^{de} \right) \left( \nabla^{(g)}{}_{(g)} R[\nabla]_{b}{}^f{}_{cf} \right) - \frac{343}{50} \text{Ttf}^{abc} \left( \nabla_{(b)}{}^{(f)} \varphi_a{}^{de} \right) \left( \nabla^{(g)}{}_{(g)} R[\nabla]_{cdef} \right) + \\
& \frac{35}{2} \text{Ttf}^{abc} \left( \nabla^{(ef)} \varphi_{ab}{}^d \right) \left( \nabla^{(g)}{}_{(g)} R[\nabla]_{cedf} \right) - \frac{189}{20} \text{Ttf}^{abc} \left( \nabla^{(e)}{}_{(e)} \varphi_{ab}{}^d \right) \left( \nabla^{(g)}{}_{(g)} R[\nabla]_{c}{}^f{}_{df} \right) + \\
& \frac{21}{10} \text{Ttf}^{abc} \left( \nabla_{(bd)} \varphi_a{}^{de} \right) \left( \nabla^{(g)}{}_{(g)} R[\nabla]_{c}{}^f{}_{ef} \right) + \frac{42}{5} \text{Ttf}^{abc} \left( \nabla_{(d)}{}^{(e)} \varphi_{ab}{}^d \right) \left( \nabla^{(g)}{}_{(g)} R[\nabla]_{c}{}^f{}_{ef} \right) - \\
& \frac{7}{5} \text{Ttf}^{abc} \left( \nabla_{(bc)} \varphi_a{}^{de} \right) \left( \nabla^{(g)}{}_{(g)} R[\nabla]_{d}{}^f{}_{ef} \right) + 7 \text{Ttf}^{abc} \left( \nabla_{(c)}{}^{(e)} \varphi_{ab}{}^d \right) \left( \nabla^{(g)}{}_{(g)} R[\nabla]_{d}{}^f{}_{ef} \right) - \\
& \frac{21}{5} \text{Ttf}^{abc} \left( \nabla^{(de)} \varphi_{abc} \right) \left( \nabla^{(g)}{}_{(g)} R[\nabla]_{d}{}^f{}_{ef} \right) - \frac{63}{20} \text{Ttf}^{abc} \left( \nabla_{(cd)} \varphi_{ab}{}^d \right) \left( \nabla^{(g)}{}_{(g)} R[\nabla]^{ef}{}_{ef} \right) + \\
& \frac{21}{8} \text{Ttf}^{abc} \left( \nabla^{(d)}{}_{(d)} \varphi_{abc} \right) \left( \nabla^{(g)}{}_{(g)} R[\nabla]^{ef}{}_{ef} \right) - \frac{14}{5} \text{Ttf}^{abc} \left( \nabla^g R[\nabla]^{de}{}_{df} \right) \left( \nabla_{(bcf)} \varphi_{aeg} \right) + \\
& \frac{7}{5} \text{Ttf}^{abc} \left( \nabla^g R[\nabla]_a{}^{def} \right) \left( \nabla_{(bcf)} \varphi_{deg} \right) - \frac{7}{50} \text{Ttf}^{abc} \left( \nabla^g \varphi^{def} \right) \left( \nabla_{(bcf)} R[\nabla]_{adeg} \right) - \\
& \frac{168}{25} \text{Ttf}^{abc} \left( \nabla_a \varphi^{def} \right) \left( \nabla_{(bcf)} R[\nabla]_d{}^g{}_{eg} \right) + \frac{14}{5} \text{Ttf}^{abc} \left( \nabla_d R[\nabla]^{defg} \right) \left( \nabla_{(bcg)} \varphi_{aef} \right) - \\
& \frac{28}{5} \text{Ttf}^{abc} \left( \nabla_e R[\nabla]^{de}{}_{df} \right) \left( \nabla_{(bcg)} \varphi_{af}{}^g \right) + \frac{14}{5} \text{Ttf}^{abc} \left( \nabla^f R[\nabla]^{de}{}_{de} \right) \left( \nabla_{(bcg)} \varphi_{af}{}^g \right) + \\
& \frac{28}{5} \text{Ttf}^{abc} \left( \nabla_e R[\nabla]_a{}^{def} \right) \left( \nabla_{(bcg)} \varphi_{df}{}^g \right) + \frac{42}{5} \text{Ttf}^{abc} \left( \nabla_a R[\nabla]^{de}{}_{df} \right) \left( \nabla_{(bcg)} \varphi_{ef}{}^g \right) + \\
& \frac{84}{5} \text{Ttf}^{abc} \left( \nabla^f R[\nabla]_a{}^d{}_{de} \right) \left( \nabla_{(bcg)} \varphi_{ef}{}^g \right) + \frac{14}{5} \text{Ttf}^{abc} \left( \nabla^f \varphi_a{}^{de} \right) \left( \nabla_{(cde)} R[\nabla]_{b}{}^g{}_{fg} \right) - \\
& \frac{14}{5} \text{Ttf}^{abc} \left( \nabla_b \varphi_a{}^{de} \right) \left( \nabla_{(cde)} R[\nabla]^{fg}{}_{fg} \right) + \frac{21}{10} \text{Ttf}^{abc} \left( \nabla^e \varphi_{ab}{}^d \right) \left( \nabla_{(cde)} R[\nabla]^{fg}{}_{fg} \right) - \\
& \frac{441}{50} \text{Ttf}^{abc} \left( \nabla^g R[\nabla]_a{}^{def} \right) \left( \nabla_{(cdf)} \varphi_{beg} \right) - \frac{56}{5} \text{Ttf}^{abc} \left( \nabla_e R[\nabla]_a{}^{def} \right) \left( \nabla_{(cdg)} \varphi_{bf}{}^g \right) + \\
& \frac{7}{5} \text{Ttf}^{abc} \left( \nabla^e \varphi_{ab}{}^d \right) \left( \nabla_{(cdg)} R[\nabla]_{e}{}^f{}_{fg} \right) + \frac{7}{5} \text{Ttf}^{abc} \left( \nabla^g R[\nabla]^{de}{}_{df} \right) \left( \nabla_{(cef)} \varphi_{abg} \right) - \\
& \frac{21}{10} \text{Ttf}^{abc} \left( \nabla^g \varphi^{def} \right) \left( \nabla_{(cef)} R[\nabla]_{adbg} \right) - \frac{42}{25} \text{Ttf}^{abc} \left( \nabla_d \varphi^{def} \right) \left( \nabla_{(cef)} R[\nabla]_a{}^g{}_{bg} \right) + \\
& \frac{42}{5} \text{Ttf}^{abc} \left( \nabla_a \varphi^{def} \right) \left( \nabla_{(cef)} R[\nabla]_{b}{}^g{}_{dg} \right) - 7 \text{Ttf}^{abc} \left( \nabla^f \varphi_a{}^{de} \right) \left( \nabla_{(cef)} R[\nabla]_{b}{}^g{}_{dg} \right) - \\
& \frac{7}{5} \text{Ttf}^{abc} \left( \nabla_d R[\nabla]^{defg} \right) \left( \nabla_{(ceg)} \varphi_{abf} \right) + \frac{161}{50} \text{Ttf}^{abc} \left( \nabla_a R[\nabla]^{defg} \right) \left( \nabla_{(ceg)} \varphi_{bdf} \right) + \\
& \frac{28}{5} \text{Ttf}^{abc} \left( \nabla^f R[\nabla]_a{}^d{}_{de} \right) \left( \nabla_{(ceg)} \varphi_{bf}{}^g \right) - \frac{49}{5} \text{Ttf}^{abc} \left( \nabla^f R[\nabla]_a{}^d{}_{be} \right) \left( \nabla_{(ceg)} \varphi_{df}{}^g \right) + \\
& \frac{217}{25} \text{Ttf}^{abc} \left( \nabla^f \varphi_a{}^{de} \right) \left( \nabla_{(ceg)} R[\nabla]_{b}{}^g{}_{df} \right) - \frac{28}{5} \text{Ttf}^{abc} \left( \nabla_b \varphi_a{}^{de} \right) \left( \nabla_{(ceg)} R[\nabla]_{d}{}^f{}_{fg} \right) +
\end{aligned}$$

$$\begin{aligned}
& \frac{21}{5} \text{Ttf}^{abc} (\nabla^g R[\nabla]^{de}{}_d{}^f) (\nabla_{(cfg)} \varphi_{abe}) + \frac{14}{5} \text{Ttf}^{abc} (\nabla_e R[\nabla]^{de}{}_d{}^f) (\nabla_{(cfg)} \varphi_{ab}{}^g) - \\
& \frac{21}{5} \text{Ttf}^{abc} (\nabla^f R[\nabla]^{de}{}_{de}) (\nabla_{(cfg)} \varphi_{ab}{}^g) - \frac{399}{50} \text{Ttf}^{abc} (\nabla^g R[\nabla]_a{}^{def}) (\nabla_{(cfg)} \varphi_{bde}) - \\
& \frac{28}{5} \text{Ttf}^{abc} (\nabla_a R[\nabla]^{de}{}_d{}^f) (\nabla_{(cfg)} \varphi_{be}{}^g) - 28 \text{Ttf}^{abc} (\nabla_d R[\nabla]_a{}^{def}) (\nabla_{(cfg)} \varphi_{be}{}^g) - \\
& \frac{112}{5} \text{Ttf}^{abc} (\nabla^f R[\nabla]_a{}^d{}_d{}^e) (\nabla_{(cfg)} \varphi_{be}{}^g) + \frac{14}{5} \text{Ttf}^{abc} (\nabla_a R[\nabla]^{de}{}_{de}) (\nabla_{(cfg)} \varphi_b{}^{fg}) + \\
& 7 \text{Ttf}^{abc} (\nabla_b R[\nabla]_a{}^{def}) (\nabla_{(cfg)} \varphi_{de}{}^g) - \frac{42}{5} \text{Ttf}^{abc} (\nabla^f R[\nabla]_a{}^d{}_b{}^e) (\nabla_{(cfg)} \varphi_{de}{}^g) + \\
& \frac{42}{5} \text{Ttf}^{abc} (\nabla_b R[\nabla]_a{}^d{}_d{}^e) (\nabla_{(cfg)} \varphi_e{}^{fg}) - 14 \text{Ttf}^{abc} (\nabla_d R[\nabla]_a{}^d{}_b{}^e) (\nabla_{(cfg)} \varphi_e{}^{fg}) - \\
& \frac{203}{50} \text{Ttf}^{abc} (\nabla^g \varphi^{def}) (\nabla_{(cfg)} R[\nabla]_{adbe}) - \frac{168}{25} \text{Ttf}^{abc} (\nabla_d \varphi^{def}) (\nabla_{(cfg)} R[\nabla]_{aeb}{}^g) - \\
& \frac{238}{25} \text{Ttf}^{abc} (\nabla_a \varphi^{def}) (\nabla_{(cfg)} R[\nabla]_{bde}{}^g) + \frac{63}{25} \text{Ttf}^{abc} (\nabla^f \varphi_a{}^{de}) (\nabla_{(cfg)} R[\nabla]_{bde}{}^g) + \\
& \frac{21}{5} \text{Ttf}^{abc} (\nabla_e R[\nabla]^{de}{}_d{}^f) (\nabla_{(c}{}^g{}_g) \varphi_{abf}) - \frac{21}{10} \text{Ttf}^{abc} (\nabla^f R[\nabla]^{de}{}_{de}) (\nabla_{(c}{}^g{}_g) \varphi_{abf}) - \\
& \frac{63}{50} \text{Ttf}^{abc} (\nabla_e R[\nabla]_a{}^{def}) (\nabla_{(c}{}^g{}_g) \varphi_{bdf}) - \frac{357}{50} \text{Ttf}^{abc} (\nabla_a R[\nabla]^{de}{}_d{}^f) (\nabla_{(c}{}^g{}_g) \varphi_{bef}) - \\
& \frac{777}{50} \text{Ttf}^{abc} (\nabla^f R[\nabla]_a{}^d{}_d{}^e) (\nabla_{(c}{}^g{}_g) \varphi_{bef}) - \frac{42}{5} \text{Ttf}^{abc} (\nabla^f R[\nabla]_a{}^d{}_b{}^e) (\nabla_{(c}{}^g{}_g) \varphi_{def}) - \\
& \frac{42}{25} \text{Ttf}^{abc} (\nabla_d \varphi^{def}) (\nabla_{(c}{}^g{}_g) R[\nabla]_{aebf}) - \frac{98}{25} \text{Ttf}^{abc} (\nabla^f \varphi_a{}^{de}) (\nabla_{(c}{}^g{}_g) R[\nabla]_{bdef}) + \\
& \frac{7}{20} \text{Ttf}^{abc} (\nabla_b \varphi_a{}^{de}) (\nabla_{(c}{}^g{}_g) R[\nabla]_d{}^f{}_{ef}) - \frac{28}{5} \text{Ttf}^{abc} (\nabla_a \varphi^{def}) (\nabla_{(def)} R[\nabla]_b{}^g{}_{cg}) + \\
& \frac{217}{25} \text{Ttf}^{abc} (\nabla^f \varphi_a{}^{de}) (\nabla_{(def)} R[\nabla]_b{}^g{}_{cg}) - \frac{161}{50} \text{Ttf}^{abc} (\nabla^f R[\nabla]_a{}^d{}_b{}^e) (\nabla_{(deg)} \varphi_{cf}{}^g) - \\
& \frac{91}{25} \text{Ttf}^{abc} (\nabla^f \varphi_a{}^{de}) (\nabla_{(deg)} R[\nabla]_{bfc}{}^g) - \frac{28}{5} \text{Ttf}^{abc} (\nabla_b \varphi_a{}^{de}) (\nabla_{(deg)} R[\nabla]_c{}^f{}_{fg}) + \\
& \frac{14}{5} \text{Ttf}^{abc} (\nabla^e \varphi_{ab}{}^d) (\nabla_{(deg)} R[\nabla]_c{}^f{}_{fg}) + \frac{98}{5} \text{Ttf}^{abc} (\nabla^g R[\nabla]_a{}^{def}) (\nabla_{(dfg)} \varphi_{bce}) + \\
& \frac{7}{5} \text{Ttf}^{abc} (\nabla_e R[\nabla]_a{}^{def}) (\nabla_{(dfg)} \varphi_{bc}{}^g) - \frac{399}{50} \text{Ttf}^{abc} (\nabla_b R[\nabla]_a{}^{def}) (\nabla_{(dfg)} \varphi_{ce}{}^g) - \\
& \frac{7}{5} \text{Ttf}^{abc} (\nabla_c \varphi_{ab}{}^d) (\nabla_{(dfg)} R[\nabla]^{ef}{}_e{}^g) + \frac{7}{5} \text{Ttf}^{abc} (\nabla^d \varphi_{abc}) (\nabla_{(dfg)} R[\nabla]^{ef}{}_e{}^g) + \\
& \frac{28}{5} \text{Ttf}^{abc} (\nabla_e R[\nabla]_a{}^{def}) (\nabla_{(d}{}^g{}_g) \varphi_{bcf}) + 7 \text{Ttf}^{abc} (\nabla^e \varphi_{ab}{}^d) (\nabla_{(d}{}^g{}_g) R[\nabla]_c{}^f{}_{ef}) - \\
& \frac{21}{20} \text{Ttf}^{abc} (\nabla_c \varphi_{ab}{}^d) (\nabla_{(d}{}^g{}_g) R[\nabla]^{ef}{}_{ef}) + \frac{49}{40} \text{Ttf}^{abc} (\nabla^d \varphi_{abc}) (\nabla_{(d}{}^g{}_g) R[\nabla]^{ef}{}_{ef}) - \\
& \frac{14}{5} \text{Ttf}^{abc} (\nabla^g R[\nabla]^{de}{}_d{}^f) (\nabla_{(efg)} \varphi_{abc}) + \frac{7}{5} \text{Ttf}^{abc} (\nabla_a R[\nabla]^{de}{}_d{}^f) (\nabla_{(efg)} \varphi_{bc}{}^g) - \\
& 7 \text{Ttf}^{abc} (\nabla^f R[\nabla]_a{}^d{}_d{}^e) (\nabla_{(efg)} \varphi_{bc}{}^g) + \frac{721}{50} \text{Ttf}^{abc} (\nabla^f R[\nabla]_a{}^d{}_b{}^e) (\nabla_{(efg)} \varphi_{cd}{}^g) + \\
& \frac{14}{5} \text{Ttf}^{abc} (\nabla_b R[\nabla]_a{}^d{}_d{}^e) (\nabla_{(efg)} \varphi_c{}^{fg}) + \frac{14}{5} \text{Ttf}^{abc} (\nabla_d R[\nabla]_a{}^d{}_b{}^e) (\nabla_{(efg)} \varphi_c{}^{fg}) - \\
& \frac{28}{5} \text{Ttf}^{abc} (\nabla^e R[\nabla]_a{}^d{}_b{}^e) (\nabla_{(efg)} \varphi_c{}^{fg}) - 7 \text{Ttf}^{abc} (\nabla_c R[\nabla]_a{}^d{}_b{}^e) (\nabla_{(efg)} \varphi_d{}^{fg}) +
\end{aligned}$$

$$\begin{aligned}
& \frac{14}{5} \text{Ttf}^{abc} (\nabla_c R[\nabla]_a^d{}_{bd}) (\nabla_{(efg)} \varphi^{efg}) - \frac{224}{25} \text{Ttf}^{abc} (\nabla_a \varphi^{def}) (\nabla_{(efg)} R[\nabla]_{bdc}{}^g) + \\
& \frac{427}{25} \text{Ttf}^{abc} (\nabla^f \varphi_a^{de}) (\nabla_{(efg)} R[\nabla]_{bdc}{}^g) - \frac{161}{50} \text{Ttf}^{abc} (\nabla_d \varphi_a^{de}) (\nabla_{(efg)} R[\nabla]_b{}^f{}_c{}^g) + \\
& \frac{399}{50} \text{Ttf}^{abc} (\nabla_b \varphi_a^{de}) (\nabla_{(efg)} R[\nabla]_c{}^f{}_d{}^g) - \frac{21}{10} \text{Ttf}^{abc} (\nabla^e \varphi_{ab}{}^d) (\nabla_{(efg)} R[\nabla]_c{}^f{}_d{}^g) - \\
& \frac{21}{5} \text{Ttf}^{abc} (\nabla^f R[\nabla]_a^d{}_{de}) (\nabla_{(efg)} \varphi_{bcf}) + \frac{56}{5} \text{Ttf}^{abc} (\nabla^f R[\nabla]_a^d{}_{be}) (\nabla_{(efg)} \varphi_{cdf}) + \\
& \frac{154}{25} \text{Ttf}^{abc} (\nabla^f \varphi_a^{de}) (\nabla_{(efg)} R[\nabla]_{bdc}{}^f) - \frac{161}{100} \text{Ttf}^{abc} (\nabla_d \varphi_a^{de}) (\nabla_{(efg)} R[\nabla]_b{}^f{}_c{}^f) - \\
& \frac{119}{25} \text{Ttf}^{abc} (\nabla_b \varphi_a^{de}) (\nabla_{(efg)} R[\nabla]_c{}^f{}_d{}^f) - \frac{161}{20} \text{Ttf}^{abc} (\nabla^e \varphi_{ab}{}^d) (\nabla_{(efg)} R[\nabla]_c{}^f{}_d{}^f) - \\
& \frac{14}{5} \text{Ttf}^{abc} (\nabla_e R[\nabla]_d{}^{de}{}_f) (\nabla_{(efg)} \varphi_{abc}) + \frac{14}{5} \text{Ttf}^{abc} (\nabla^f R[\nabla]^{de}{}_{de}) (\nabla_{(efg)} \varphi_{abc}) + \\
& \frac{7}{5} \text{Ttf}^{abc} (\nabla_a R[\nabla]_d{}^{de}{}_f) (\nabla_{(efg)} \varphi_{bce}) + \frac{126}{5} \text{Ttf}^{abc} (\nabla_d R[\nabla]_a{}^{def}) (\nabla_{(efg)} \varphi_{bce}) + \\
& \frac{91}{5} \text{Ttf}^{abc} (\nabla^f R[\nabla]_a^d{}_{de}) (\nabla_{(efg)} \varphi_{bce}) - \frac{21}{10} \text{Ttf}^{abc} (\nabla_a R[\nabla]^{de}{}_{de}) (\nabla_{(efg)} \varphi_{bc}{}^f) - \\
& \frac{7}{5} \text{Ttf}^{abc} (\nabla_e R[\nabla]_a^d{}_{de}) (\nabla_{(efg)} \varphi_{bc}{}^f) + \frac{42}{5} \text{Ttf}^{abc} (\nabla^f R[\nabla]_a^d{}_{be}) (\nabla_{(efg)} \varphi_{cde}) - \\
& \frac{343}{50} \text{Ttf}^{abc} (\nabla_b R[\nabla]_a^d{}_{de}) (\nabla_{(efg)} \varphi_{ce}{}^f) + \frac{623}{50} \text{Ttf}^{abc} (\nabla_d R[\nabla]_a^d{}_{be}) (\nabla_{(efg)} \varphi_{ce}{}^f) + \\
& \frac{77}{50} \text{Ttf}^{abc} (\nabla^e R[\nabla]_a^d{}_{bd}) (\nabla_{(efg)} \varphi_{ce}{}^f) - \frac{112}{25} \text{Ttf}^{abc} (\nabla_a \varphi^{def}) (\nabla_{(efg)} R[\nabla]_{bdce}) + \\
& \frac{77}{25} \text{Ttf}^{abc} (\nabla^f \varphi_a^{de}) (\nabla_{(efg)} R[\nabla]_{bdce}) - \frac{224}{25} \text{Ttf}^{abc} (\nabla_b \varphi_a^{de}) (\nabla_{(efg)} R[\nabla]_{cde}{}^f) + \\
& \frac{98}{75} \text{Ttf}^{abc} (\nabla_d \varphi_{ab}{}^d) (\nabla_{(efg)} R[\nabla]_c{}^e{}_f) + \frac{77}{5} \text{Ttf}^{abc} (\nabla^e \varphi_{ab}{}^d) (\nabla_{(efg)} R[\nabla]_c{}^f{}_de) - \\
& \frac{518}{75} \text{Ttf}^{abc} (\nabla_c \varphi_{ab}{}^d) (\nabla_{(efg)} R[\nabla]_d{}^e{}_f) + \frac{14}{5} \text{Ttf}^{abc} (\nabla^d \varphi_{abc}) (\nabla_{(efg)} R[\nabla]_d{}^e{}_f) + \\
& \frac{14}{5} R[\nabla]^{de}{}_d{}^f \text{Ttf}^{abc} (\nabla_{(abcg)} \varphi_{ef}{}^g) + \frac{3}{25} \varphi^{abc} \text{Ttf}^{def} (\nabla_{(bcef)} R[\nabla]_a{}^g{}_dg) - \\
& \frac{28}{5} R[\nabla]^{de}{}_d{}^f \text{Ttf}^{abc} (\nabla_{(bcfg)} \varphi_{ae}{}^g) + \frac{14}{5} R[\nabla]^{de}{}_{de} \text{Ttf}^{abc} (\nabla_{(bcfg)} \varphi_a{}^fg) + \\
& \frac{42}{5} R[\nabla]_a{}^{def} \text{Ttf}^{abc} (\nabla_{(bcfg)} \varphi_{de}{}^g) + \frac{63}{5} R[\nabla]_a^d{}_{de} \text{Ttf}^{abc} (\nabla_{(bcfg)} \varphi_e{}^fg) - \\
& \frac{14}{5} R[\nabla]^{de}{}_d{}^f \text{Ttf}^{abc} (\nabla_{(bcg)} \varphi_{ae}{}^f) - \frac{28}{25} \varphi^{abc} \text{Ttf}^{def} (\nabla_{(cdef)} R[\nabla]_a{}^g{}_bg) - \\
& \frac{84}{5} R[\nabla]_a{}^{def} \text{Ttf}^{abc} (\nabla_{(cdfg)} \varphi_{be}{}^g) + \frac{14}{5} R[\nabla]^{de}{}_d{}^f \text{Ttf}^{abc} (\nabla_{(cefg)} \varphi_{ab}{}^g) + \\
& \frac{28}{5} R[\nabla]_a^d{}_{de} \text{Ttf}^{abc} (\nabla_{(cefg)} \varphi_b{}^fg) - \frac{42}{5} R[\nabla]_a^d{}_{be} \text{Ttf}^{abc} (\nabla_{(cefg)} \varphi_d{}^fg) + \\
& \frac{14}{5} R[\nabla]_a^d{}_{bd} \text{Ttf}^{abc} (\nabla_{(cefg)} \varphi^{efg}) + \frac{168}{25} \varphi^{abc} \text{Ttf}^{def} (\nabla_{(cefg)} R[\nabla]_{adb}{}^g) + \\
& \frac{21}{5} \varphi^{abc} \text{Ttf}_a{}^{de} (\nabla_{(ceg)} R[\nabla]_b{}^f{}_df) + \frac{28}{5} R[\nabla]^{de}{}_d{}^f \text{Ttf}^{abc} (\nabla_{(cfg)} \varphi_{abe}) - \\
& \frac{21}{5} R[\nabla]^{de}{}_{de} \text{Ttf}^{abc} (\nabla_{(cfg)} \varphi_{ab}{}^f) - \frac{56}{5} R[\nabla]_a{}^{def} \text{Ttf}^{abc} (\nabla_{(cfg)} \varphi_{bde}) -
\end{aligned}$$

$$\begin{aligned}
& \frac{112}{5} R[\nabla]_a^d{}^e \text{Ttf}^{abc} \left( \nabla_{(cf}^g \varphi_{b e}^f \right) - \frac{42}{5} R[\nabla]_a^d{}^e \text{Ttf}^{abc} \left( \nabla_{(cf}^g \varphi_{de}^f \right) - \\
& \frac{36}{5} \varphi^{abc} \text{Ttf}^{def} \left( \nabla_{(cf}^g R[\nabla]_{adbe} \right) + \frac{161}{50} \varphi^{abc} \text{Ttf}_a^{de} \left( \nabla_{(defg)} R[\nabla]_b^f{}^c{}^g \right) - \\
& \frac{259}{100} \varphi^{abc} \text{Ttf}_a^{de} \left( \nabla_{(de}^g R[\nabla]_b^f{}^c{}^f \right) + \frac{98}{5} R[\nabla]_a^{def} \text{Ttf}^{abc} \left( \nabla_{(df}^g \varphi_{bce} \right) - \\
& \frac{203}{75} \varphi^{abc} \text{Ttf}_{ab}^d \left( \nabla_{(df}^g R[\nabla]_c^e{}^f \right) - \frac{14}{5} R[\nabla]^{def}{}_d \text{Ttf}^{abc} \left( \nabla_{(ef}^g \varphi_{abc} \right) - \\
& \frac{28}{5} R[\nabla]_a^d{}^e \text{Ttf}^{abc} \left( \nabla_{(ef}^g \varphi_{bc}^f \right) + \frac{56}{5} R[\nabla]_a^d{}^e \text{Ttf}^{abc} \left( \nabla_{(ef}^g \varphi_{cd}^f \right) - \\
& \frac{14}{5} R[\nabla]_a^d{}^e \text{Ttf}^{abc} \left( \nabla_{(ef}^g \varphi_c^{ef} \right) + \frac{7}{5} \varphi^{abc} \text{Ttf}_a^{de} \left( \nabla_{(ef}^g R[\nabla]_{bdc}^f \right) + \\
& \frac{7}{5} R[\nabla]^{de}{}_{de} \text{Ttf}^{abc} \left( \nabla_{(f}^g \varphi_{abc} \right) + \frac{91}{10} R[\nabla]_a^d{}^e \text{Ttf}^{abc} \left( \nabla_{(f}^g \varphi_{bce} \right) + \\
& \frac{21}{5} R[\nabla]_a^d{}^e \text{Ttf}^{abc} \left( \nabla_{(f}^g \varphi_{cde} \right) - \frac{219}{25} \varphi^{abc} \text{Ttf}_{ab}^d \left( \nabla_{(f}^g R[\nabla]_c^e{}_{de} \right) + \\
& \frac{171}{100} \varphi^{abc} \text{Ttf}_{abc} \left( \nabla_{(f}^g R[\nabla]^{de}{}_{de} \right) - \frac{2}{5} \text{Ttf}^{abc} \left( \nabla_{(abcdef)} \varphi^{def} \right) + \\
& \frac{12}{5} \text{Ttf}^{abc} \left( \nabla_{(bcde}^f \varphi_a^{de} \right) - 3 \text{Ttf}^{abc} \left( \nabla_{(cd}^e{}^f \varphi_{ab}^d \right) + \text{Ttf}^{abc} \left( \nabla_{(de}^d{}^e{}^f \varphi_{abc} \right) = 0
\end{aligned}$$

## System requirements

This notebook has been written and executed on *Mathematica* 9:

**System`\$Version**

9.0 for Mac OS X x86 (64-bit) (January 24, 2013)

It requires only the *xAct* collection of packages, which can be obtained for free from [www.xact.es](http://www.xact.es).

The following versions of the various packages have been used to execute this notebook:

**xAct`xPerm`\$Version**

{1.2.1, {2014, 2, 15}}

**xAct`xTensor`\$Version**

{1.1.0, {2014, 2, 23}}

**xAct`xTras`\$Version**

{1.3.3, {2014, 3, 31}}

All in all, the total running time of this notebook is about one day.

## Calculation

### I. Initialization

#### I.0 Description

In this second we'll initialize the packages, define the manifold and tensors, and define some func-

tions that will be used throughout the notebook.

## I.1 Package and tensors

First of all, we load the xTras package (<http://www.xact.es/xtras/>).

```
In[1]:= << xAct`xTras`

-----

Package xAct`xPerm` version 1.2.1, {2014, 2, 15}
Copyright (C) 2003-2014, Jose M. Martin-Garcia, under the General Public License.
Connecting to external mac executable...
Connection established.

-----

Package xAct`xTensor` version 1.1.0, {2014, 2, 23}
Copyright (C) 2002-2014, Jose M. Martin-Garcia, under the General Public License.

-----

Package xAct`xPert` version 1.0.4, {2014, 2, 15}
Copyright (C) 2005-2014, David Brizuela, Jose M. Martin-Garcia
and Guillermo A. Mena Marugan, under the General Public License.
** Variable $PrePrint assigned value ScreenDollarIndices
** Variable $CovDFormat changed from Prefix to Postfix
** Option AllowUpperDerivatives of ContractMetric changed from False to True
** Option MetricOn of MakeRule changed from None to All
** Option ContractMetrics of MakeRule changed from False to True

-----

Package xAct`Invar` version 2.0.5, {2014, 2, 15}
Copyright (C) 2006-2014, J. M. Martin-Garcia,
D. Yllanes and R. Portugal, under the General Public License.
** DefConstantSymbol: Defining constant symbol sigma.
** DefConstantSymbol: Defining constant symbol dim.
** Option CurvatureRelations of DefCovD changed from True to False
** Variable $CommuteCovDsOnScalars changed from True to False

-----

Package xAct`xCoba` version 0.8.1, {2014, 2, 15}
Copyright (C) 2005-2014, David Yllanes and
Jose M. Martin-Garcia, under the General Public License.

-----

Package xAct`SymManipulator` version 0.9.0, {2014, 1, 24}
Copyright (C) 2011-2014, Thomas Bäckdahl, under the General Public License.

-----

Package xAct`xTras` version 1.3.3, {2014, 3, 31}
Copyright (C) 2012-2014, Teake Nutma, under the General Public License.
** Variable $CovDFormat changed from Postfix to Prefix
```



**\*\* Option CurvatureRelations of DefCovD changed from False to True**

-----

These packages come with ABSOLUTELY NO WARRANTY; for details type  
Disclaimer[]. This is free software, and you are welcome to redistribute  
it under certain conditions. See the General Public License for details.

-----

We'll be dealing with expressions that have a large number of constants, whereupon Simplify will take a lot of time. Therefore we set the method of simplifying overall coefficients of tensorial terms in CollectTensors to Expand.

In[2]:= **SetOptions[CollectTensors, SimplifyMethod → Expand]**

Out[2]= {CollectMethod → Default, SimplifyMethod → Expand,  
RemoveTensorWrapper → True, Verbose → False}

Define a 4-dimensional manifold with indices a,b,c,...k,l.

In[3]:= **DefManifold[M, 4, IndexRange[a, l]]**

**\*\* DefManifold:** Defining manifold M.

**\*\* DefVBundle:** Defining vbundle TangentM.

Define a Lorentzian metric on the manifold whose derivatives can be symmetrized.

In[4]:= **DefMetric[-1, metric[-a, -b], CD, PrintAs → "g",  
CurvatureRelations -> False, SymCovDQ → True]**

```

** DefTensor: Defining symmetric metric tensor metric[-a, -b].
** DefTensor: Defining antisymmetric tensor epsilonmetric[-a, -b, -c, -d].
** DefTensor: Defining tetrametric Tetrametric[-a, -b, -c, -d].
** DefTensor: Defining tetrametric Tetrametric†[-a, -b, -c, -d].
** DefCovD: Defining covariant derivative CD[-a].
** DefTensor: Defining vanishing torsion tensor TorsionCD[a, -b, -c].
** DefTensor: Defining symmetric Christoffel tensor ChristoffelCD[a, -b, -c].
** DefTensor: Defining Riemann tensor RiemannCD[-a, -b, -c, -d].
** DefTensor: Defining symmetric Ricci tensor RicciCD[-a, -b].
** DefTensor: Defining Ricci scalar RicciScalarCD[].
** DefTensor: Defining symmetric Einstein tensor EinsteinCD[-a, -b].
** DefTensor: Defining Weyl tensor WeylCD[-a, -b, -c, -d].
** DefTensor: Defining symmetric TFRicci tensor TFRicciCD[-a, -b].
** DefTensor: Defining Kretschmann scalar KretschmannCD[].
** DefCovD: Computing RiemannToWeylRules for dim 4
** DefCovD: Computing RicciToTFRicci for dim 4
** DefCovD: Computing RicciToEinsteinRules for dim 4
** DefTensor: Defining symmetrized Riemann tensor SymRiemannCD[-a, -b, -c, -d].
** DefTensor: Defining symmetric Schouten tensor SchoutenCD[-a, -b].
** DefTensor: Defining
    symmetric cosmological Schouten tensor SchoutenCCCD[LI[___], -a, -b].
** DefTensor: Defining
    symmetric cosmological Einstein tensor EinsteinCCCD[LI[___], -a, -b].
** DefCovD: Defining covariant derivative CD[-a]. to be symmetrizable
** DefTensor: Defining weight +2 density Detmetric[]. Determinant.
** DefParameter: Defining parameter PerturbationParametermetric.
** DefTensor: Defining tensor Perturbationmetric[LI[order], -a, -b].

```

Define a dilaton that we'll use to do Weyl rescalings.

```

In[5]:= DefTensor[Ω[___], M]

** DefTensor: Defining tensor Ω[___].

```

Define a cosmological constant.

```

In[384]:= DefConstantSymbol[Λ]

** DefConstantSymbol: Defining constant symbol Λ.

```

Define the spin-3 field  $\varphi_{abc}$ :

```

In[6]:= DefTensor[phi[-a, -b, -c], M, Symmetric[{-a, -b, -c}], PrintAs -> "φ"]

** DefTensor: Defining tensor phi[-a, -b, -c].

```

Set it to be traceless:

```

In[7]:= phi[___, a_, ___, b_, ___] /; PairQ[a, b] = 0

```

```

Out[7]= 0

```

Define an auxiliary symmetry rank-3 tensor T3. We can use this to contract equations of motion, which will reduce the number of terms by a factor of 3! at most.

```
In[8]:= DefTensor[T3[-a, -b, -c], M, Symmetric[{-a, -b, -c}], PrintAs -> "T"]
** DefTensor: Defining tensor T3[-a, -b, -c].
```

Deduce the traceless projector on symmetric rank-3 tensors, which we'll call TFprojector:

```
In[9]:= MakeTraceless[T3[d, e, f]] // ExpandSym
TFprojector = VarD[T3[a, b, c]][%] // ToCanonical
```

```
Out[9]= T^{def} + \frac{1}{12} (-g^{ef} T^{da}_a - g^{fe} T^{da}_a - g^{df} T^{ea}_a - g^{fd} T^{ea}_a - g^{de} T^{fa}_a - g^{ed} T^{fa}_a)
```

VarD::nouse : Attempting to apply VarD on a non-scalar expression.

```
Out[10]= \frac{1}{6} \delta_a^f \delta_b^e \delta_c^d + \frac{1}{6} \delta_a^e \delta_b^f \delta_c^d + \frac{1}{6} \delta_a^f \delta_b^d \delta_c^e +
\frac{1}{6} \delta_a^d \delta_b^f \delta_c^e + \frac{1}{6} \delta_a^e \delta_b^d \delta_c^f + \frac{1}{6} \delta_a^d \delta_b^e \delta_c^f - \frac{1}{18} \delta_c^f g_{ab} g^{de} -
\frac{1}{18} \delta_b^f g_{ac} g^{de} - \frac{1}{18} \delta_a^f g_{bc} g^{de} - \frac{1}{18} \delta_c^e g_{ab} g^{df} - \frac{1}{18} \delta_b^e g_{ac} g^{df} -
\frac{1}{18} \delta_a^e g_{bc} g^{df} - \frac{1}{18} \delta_c^d g_{ab} g^{ef} - \frac{1}{18} \delta_b^d g_{ac} g^{ef} - \frac{1}{18} \delta_a^d g_{bc} g^{ef}
```

Also define another auxiliary symmetric rank-3 tensor T3TF, which is also traceless:

```
In[11]:= DefTensor[T3TF[-a, -b, -c], M, Symmetric[{-a, -b, -c}], PrintAs -> "Ttf"]
** DefTensor: Defining tensor T3TF[-a, -b, -c].
```

```
In[12]:= T3TF[___, a_, ___, b_, ___] /; PairQ[a, b] = 0
```

```
Out[12]= 0
```

A double-check that the projector is correct:

```
In[13]:= TFprojector T3TF[-d, -e, -f] // CollectTensors
```

```
Out[13]= Ttf_{abc}
```

Define the gauge parameter of the spin-3 transformations:

```
In[14]:= DefTensor[xi[-a, -b], M, Symmetric[{-a, -b}], PrintAs -> "\xi"]
** DefTensor: Defining tensor xi[-a, -b].
```

It is also effectively traceless:

```
In[15]:= xi[a_, b_] /; PairQ[a, b] := 0
```

```
In[16]:= xi[a, -a]
```

```
Out[16]= 0
```

Make a short-cut to a private Invar function that converts Ricci tensors and scalars to contractions of Riemann tensors:

```
In[17]:= RicciToRiemann = xAct`Invar`Private`RicciToRiemann[#, CD] &;
```

## I.2 Code for saving expressions to disk

This subsection contains code for writing tensorial expressions to file, and for loading tensorial expressions from a file.

This is very convenient for saving the results of long calculations.

This is not general-purpose code; at the moment it only attempts to replace dollar indices with regular indices, and it saves the definitions of any constant symbol appearing in expressions.

All expressions will be saved to a separate subdirectory called “notebookfilename + calculations”:

```
In[18]:= $SaveDirectory = FileNameJoin[  

         {NotebookDirectory[], FileName@NotebookFileName[] <> " calculations"}];
```

If that directory doesn't exist, create it:

```
In[19]:= If[! DirectoryQ[$SaveDirectory],  

           CreateDirectory[$SaveDirectory]  

         ];
```

Get a list of indices that will be used to replace dollar indices in expressions:

```
In[20]:= indicesList = IndexList @@ GetIndicesOfVBundle[TangentM, 22]
```

```
Out[20]:= {a, b, c, d, e, f, g, h, i, j,  

          k, 1, 11, 12, 13, 14, 15, 16, 17, 18, 19, 110}
```

Now come the main functions, **TensorPut** and **TensorGet**.

```
In[21]:= ClearAll[TensorPut];
```

```
TensorPut::usage =
  "TensorPut[symbol] saves the value of symbol to 'symbol.m' in the
  $SaveDirectory iff symbol has a value and the file does not
  exists before. It also makes an effort to save any constant
  variables in symbol, and to replace its dummy indices. It returns
  the name of the file saved to if succesful, or Null otherwise.";
TensorPut::exists = "Won't save `1` to `2` because the file already exists.";
TensorPut::novalue = "Won't save `1` because it doesn't have a value.";

Options[TensorPut] ^= {"Overwrite" -> False};

ReplaceDummiesList[expr_List] := ReplaceDummiesList /@ expr;
ReplaceDummiesList[expr_] :=
  ReplaceDummies[
    expr,
    Complement[
      indicesList,
      UpIndex /@ IndicesOf[Free][expr]
    ]
  ];

TensorPut[symbol_Symbol, OptionsPattern[]] := With[{
  (* Name of the file to save to. *)
  filename = FileNameJoin[
    {$SaveDirectory, StringJoin[ToString[HoldForm@symbol], ".m"]}
  ],
  (* Check if the file exists. *)
  If[
    ! FileExistsQ[filename] || OptionValue["Overwrite"]
  ],
  (* If the file does not exists, write out the data. *)
  (* The Block is to prevent DefConstantSymbolList from evaluating. *)
  Block[{DefConstantSymbolList, SetUsageMessage},
    Put[
      (* Save a list of constants in the symbol value. *)
      DefConstantSymbolList[{#, PrintAs[#]} & /@ ConstantSymbolsOf[symbol]],
      (* Replace dummies with non-dollar indices. *)
      ReplaceDummiesList[symbol],
      filename
    ]
  ];
  (* Return the name of the file saved to. *)
  FileNameTake[filename, -1]
},
  (* If the file does already exists,
  give a warning message and return Null. *)
  Message[TensorPut::exists, ToString[HoldForm@symbol], filename];
  Null
];

TensorPut[symbol_Symbol] /; ! ValueQ[symbol] :=
  Message[TensorPut::novalue, ToString[HoldForm@symbol]];
SetAttributes[TensorPut, HoldFirst];
TensorPut[list_List] := ReleaseHold@Map[TensorPut, Hold@list, {2}]
```

```

In[32]:= TensorGet::usage =
  "TensorGet[symbol] set the value of symbol to the output of the file
  'symbol.m' in $SaveDirectory iff symbol doesn't have a value.";
TensorGet::value = "Won't load definitions for `1`
  because it already has a value.";
TensorGet::nofile = "Can't load definitions for `1`
  because no file can be found.";
TensorGet[symbol_Symbol] := Block[{
  filenames = FileNames[ToString[HoldForm@symbol] ~~ ".m", {$SaveDirectory}],
  SetUsageMessage = (MessageName[symbol, "usage"] = #) &
},
If[Length@filenames === 0,
  Message[TensorGet::nofile, ToString[HoldForm@symbol]];
  Return[$Failed]
];
If[
  # != $Failed,
  symbol = #;
  FileNameTake[First@filenames, -1],
  $Failed
] & @Get@First@filenames
];
TensorGet[symbol_Symbol] /; ValueQ[symbol] :=
  Message[TensorGet::value, ToString[HoldForm@symbol]];
SetAttributes[TensorGet, HoldFirst];
TensorGet[list_List] := ReleaseHold@Map[TensorGet, Hold@list, {2}]

In[39]:= DefConstantSymbolList[list : {{_, _} ...}] := DefConstantSymbolList /@ list;
DefConstantSymbolList[{constant_, printas_}] := Block[
  {$DefInfoQ = False},
  Quiet[
    DefConstantSymbol[constant, PrintAs -> printas], {ValidateSymbol::used}
  ]
];

```

### I.3 Linear in Riemann tensors

Because we work linearly in the Riemann tensor, any n-fold derivative of the Riemann tensor is automatically symmetric and lives in the  $\{2+n,2\}$  Young tableaux.

This function automatically sets any square of the Riemann tensor to zero:

```

In[41]:= SetLinearRiemann[] :=
  (
    CD[a__] @ CD[b__] [x_RiemannCD] := CD[a, b] [x];
    RiemannCD /: RiemannCD[x__] * RiemannCD[y__] = 0;
    RiemannCD /: CD[__] @ RiemannCD[__] * RiemannCD[__] = 0;
    CD /: CD[x__] @ RiemannCD[__] * CD[y__] @ RiemannCD[__] = 0;
  );

```

This function removes the definitions of the function above:

```

In[42]:= ClearLinearRiemann[] :=
  (
    CD[a__] @ CD[b__] [x_RiemannCD] =.;
    RiemannCD /: RiemannCD[x__] * RiemannCD[y__] =.;
    RiemannCD /: CD[__] @ RiemannCD[__] * RiemannCD[__] =.;
    CD /: CD[x__] @ RiemannCD[__] * CD[y__] @ RiemannCD[__] =.;
  );

```

```

In[43]:= SetLinearRiemann[]

```

Test:

```
In[44]:= CD[a]@CD[b]@CD[c]@RiemannCD[e, f, g, h]
```

```
Out[44]=  $\nabla^{(abc)} R[\nabla]^{efgh}$ 
```

Test:

```
In[45]:= CD[a]@RiemannCD[b, c, d, e] RiemannCD[f, g, h, i]
RiemannCD[b, c, d, e] RiemannCD[f, g, h, i]
CD[a]@RiemannCD[b, c, d, e] CD[j]@RiemannCD[f, g, h, i]
```

```
Out[45]= 0
```

```
Out[46]= 0
```

```
Out[47]= 0
```

## I.4 Young tableaux computation

In this subsection we precompute the projection of the n-fold derivative on the Riemann tensor onto the  $\{2+n,2\}$  Young tableaux. Going to this basis automatically projects out any Bianchi identities.

Zeroth derivative:

```
RiemannCD[a, b, c, d]
YoungProject[%, {{a, c}, {b, d}}]
ypscdrRule0 = MakeRule@Evaluate@{%%, %}
%% - (%% /. %) // ToCanonical
```

```
R[ $\nabla$ ]abcd
```

$$\frac{2}{3} R[\nabla]^{abcd} + \frac{1}{3} R[\nabla]^{acbd} - \frac{1}{3} R[\nabla]^{adbc}$$

$$\left\{ \text{HoldPattern}[R[\nabla]^{\underline{abcd}}] \rightarrow \text{Module}\left[\{\}, \frac{2}{3} R[\nabla]^{abcd} + \frac{1}{3} R[\nabla]^{acbd} - \frac{1}{3} R[\nabla]^{adbc}\right] \right\}$$

```
0
```

First derivative:

```

CD[e]@RiemannCD[a, b, c, d]
YoungProject[%, {{a, c, e}, {b, d}}]
ypscdrRule1 = MakeRule@Evaluate@{%%, %}
%% - (%% /. %) // ToCanonical

```

$\nabla^e R[\nabla]^{abcd}$

$$\begin{aligned}
& \frac{1}{12} (\nabla^a R[\nabla]^{bcde}) - \frac{1}{12} (\nabla^a R[\nabla]^{bdce}) - \frac{1}{6} (\nabla^a R[\nabla]^{becd}) - \\
& \frac{1}{12} (\nabla^b R[\nabla]^{acde}) + \frac{1}{12} (\nabla^b R[\nabla]^{adce}) + \frac{1}{6} (\nabla^b R[\nabla]^{aecd}) - \frac{1}{6} (\nabla^c R[\nabla]^{abde}) - \\
& \frac{1}{12} (\nabla^c R[\nabla]^{adbe}) + \frac{1}{12} (\nabla^c R[\nabla]^{aebd}) + \frac{1}{6} (\nabla^d R[\nabla]^{abce}) + \frac{1}{12} (\nabla^d R[\nabla]^{acbe}) - \\
& \frac{1}{12} (\nabla^d R[\nabla]^{aebc}) + \frac{1}{3} (\nabla^e R[\nabla]^{abcd}) + \frac{1}{6} (\nabla^e R[\nabla]^{acbd}) - \frac{1}{6} (\nabla^e R[\nabla]^{adbc})
\end{aligned}$$

$\{ \text{HoldPattern}[\nabla^e R[\nabla]^{\underline{abcd}}] \rightarrow$

$$\begin{aligned}
& \text{Module}\left[\{\}, \frac{1}{12} (\nabla^a R[\nabla]^{bcde}) - \frac{1}{12} (\nabla^a R[\nabla]^{bdce}) - \frac{1}{6} (\nabla^a R[\nabla]^{becd}) - \right. \\
& \frac{1}{12} (\nabla^b R[\nabla]^{acde}) + \frac{1}{12} (\nabla^b R[\nabla]^{adce}) + \frac{1}{6} (\nabla^b R[\nabla]^{aecd}) - \frac{1}{6} (\nabla^c R[\nabla]^{abde}) - \\
& \frac{1}{12} (\nabla^c R[\nabla]^{adbe}) + \frac{1}{12} (\nabla^c R[\nabla]^{aebd}) + \frac{1}{6} (\nabla^d R[\nabla]^{abce}) + \frac{1}{12} (\nabla^d R[\nabla]^{acbe}) - \\
& \left. \frac{1}{12} (\nabla^d R[\nabla]^{aebc}) + \frac{1}{3} (\nabla^e R[\nabla]^{abcd}) + \frac{1}{6} (\nabla^e R[\nabla]^{acbd}) - \frac{1}{6} (\nabla^e R[\nabla]^{adbc}) \right] \}
\end{aligned}$$

0

Second derivative:

```

CD[e, f]@RiemannCD[a, b, c, d]
YoungProject[%, {{a, c, e, f}, {b, d}}];
ypscdrRule2 = MakeRule@Evaluate@{%%, %};
%% - (%% /. %) // ToCanonical

```

$\nabla^{(ef)} R[\nabla]^{abcd}$

0

Third derivative:

```

CD[e, f, g]@RiemannCD[a, b, c, d]
YoungProject[%, {{a, c, e, f, g}, {b, d}}];
ypscdrRule3 = MakeRule@Evaluate@{%%, %};
%% - (%% /. %) // ToCanonical

```

$\nabla^{(efg)} R[\nabla]^{abcd}$

\$Aborted

Fourth derivative:

```

CD[e, f, g, h]@RiemannCD[a, b, c, d]
YoungProject[%, {{a, c, e, f, g, h}, {b, d}}];
ypscdrRule4 = MakeRule@Evaluate@{%%, %};

```

$\nabla^{(efgh)} R[\nabla]^{abcd}$

Fifth derivative:



```

CD[e, f, g, h, i]@RiemannCD[a, b, c, d]
YoungProject[%, {{a, c, e, f, g, h, i}, {b, d}}];
ypscdrRule5 = MakeRule@Evaluate@{%%, %};
 $\nabla^{(efghi)} R[\nabla]^{abcd}$ 

```

Combine all rules:

```

ypriemannRules = Join[
  ypscdrRule0,
  ypscdrRule1,
  ypscdrRule2,
  ypscdrRule3,
  ypscdrRule4,
  ypscdrRule5
];

```

And save them:

```

TensorPut[ypriemannRules]
ypriemannRules.m

```

## I.5 Young tableaux function

This subsection contains a function that projects Riemann tensors onto the Young tableaux we computed in the previous subsection.

Load the projection rules:

```
In[48]:= TensorGet[ypriemannRules]
```

```
Out[48]:= ypriemannRules.m
```

Check that we loaded the correct rule:

```
In[49]:= First /@ ypriemannRules
```

```

Out[49]= {HoldPattern[R[ $\nabla$ ]abcd], HoldPattern[ $\nabla^e$  R[ $\nabla$ ]abcd],
  HoldPattern[ $\nabla^{(ef)}$  R[ $\nabla$ ]abcd], HoldPattern[ $\nabla^{(efg)}$  R[ $\nabla$ ]abcd],
  HoldPattern[ $\nabla^{(efgh)}$  R[ $\nabla$ ]abcd], HoldPattern[ $\nabla^{(efghi)}$  R[ $\nabla$ ]abcd]}

```

```
In[50]:= First@ypriemannRules
```

```

Out[50]= HoldPattern[R[ $\nabla$ ]abcd] :> Module[{ },  $\frac{2}{3} R[\nabla]^{abcd} + \frac{1}{3} R[\nabla]^{acbd} - \frac{1}{3} R[\nabla]^{adbc}$ ]

```

The Weyl tensor and its derivatives live in the same tableaux, so we can simply use the rules for the Riemann tensor if we replace any occurrence of RiemannCD with WeylCD.

```
In[51]:= ypweylRules = ypriemannRules /. RiemannCD -> WeylCD;
```

```
In[52]:= First /@ ypweylRules
```

```

Out[52]= {HoldPattern[W[ $\nabla$ ]abcd], HoldPattern[ $\nabla^e$  W[ $\nabla$ ]abcd],
  HoldPattern[ $\nabla^{(ef)}$  W[ $\nabla$ ]abcd], HoldPattern[ $\nabla^{(efg)}$  W[ $\nabla$ ]abcd],
  HoldPattern[ $\nabla^{(efgh)}$  W[ $\nabla$ ]abcd], HoldPattern[ $\nabla^{(efghi)}$  W[ $\nabla$ ]abcd]}

```

```
In[53]:= First@ypweylRules
```

```
Out[53]= HoldPattern[W[∇] abcd] := Module[{ },  $\frac{2}{3} W[\nabla]^{abcd} + \frac{1}{3} W[\nabla]^{acbd} - \frac{1}{3} W[\nabla]^{adbc}$ ]
```

This function does the actual projecting:

```
In[54]:= ClearAll[ProjectRiemanns];
ProjectRiemanns[list_List] :=
  MapTimed[ProjectRiemanns, list];
ProjectRiemanns[x_] :=
  CollectTensors[
    MapTimedTensors[
      CollectTensors[# /. ypriemannRules /. ypweylRules] &,
      x
    ],
    CollectMethod → Identity
  ];
```

Here's a small test. This should be zero:

```
In[57]:= CD[b, c, d, f]@CD[a]@RicciToRiemann@EinsteinToRicci[EinsteinCD[-a, -e]]
% // ProjectRiemanns
```

```
Out[57]=  $\nabla^{(bcdfa)} R[\nabla]_{age}^g - \frac{1}{2} g_{ea} \left( \nabla^{(bcdfa)} R[\nabla]_{gh}^{gh} \right)$ 
```

```
Out[58]= 0
```

And indeed it is.

## 2 Weyl gravity

### 2.0 Description

In this section we derive the equations of motion of Weyl gravity, namely the vanishing of the Bach tensor.

#### 2.1 Action and equations of motion

The Weyl action is quadratic in Riemann tensors, so we need to clear the definitions that make everything linear in Riemanns.

```
ClearLinearRiemann[]
```

We'll also re-enable the curvature relations for the moment.

```
SetCurvatureRelations[CD]
```

```
Rules {17, 18} have been declared as DownValues for RicciCD.
```

```
Rules {1, 2, 3, 4, 5, 6, 7, 8, 9, 10, <<6>>}
have been declared as UpValues for RicciCD.
```

```
Rules {1, 2, 3, 4, 5, 6, 7, 8, 9, 10, <<4>>}
have been declared as DownValues for RiemannCD.
```

```
Rules {1, 2, 3, 4, 5, 6, 7, 8, 9, 10, <<14>>}
have been declared as DownValues for SymRiemannCD.
```

The action for Weyl gravity is:

**S0 = WeylCD[a, b, c, d] WeylCD[-a, -b, -c, -d]**

$W[\nabla]_{abcd} W[\nabla]^{abcd}$

And its equations of motion read ...

**eom0 = VarL[metric[-a, -b], CD][S0] // RiemannToWeyl // SymmetrizeCovDs // CollectTensors**

$-2 R[\nabla]^{cd} W[\nabla]_c^a W[\nabla]_d^b - 2 W[\nabla]^{acde} W[\nabla]_c^b W[\nabla]_{cde} +$   
 $\frac{1}{2} g^{ab} W[\nabla]_{cdef} W[\nabla]^{cdef} - 4 (\nabla_{(cd} W[\nabla]^{acbd})$

This is not exactly the Bach tensor; there are some Weyl squared terms still present. These are actually zero, as can be shown by constructing all Dimensional Dependent Identities for Weyl squared terms with two free indices:

**eom0ddis = ConstructDDIs[IndexFree[WeylCD^2], {a, b}, Symmetric[{a, b}]]**

**\*\* DefTensor:** Defining basic dimensional dependent identity  
 BasicDDICD4[-a, -b, -c, -d, -e, -f, -g, -h, -i, -j].

$\left\{ W[\nabla]^{acde} W[\nabla]_c^b W[\nabla]_{cde} - \frac{1}{4} g^{ab} W[\nabla]_{cdef} W[\nabla]^{cdef}, \right.$   
 $W[\nabla]^{acde} W[\nabla]_c^b W[\nabla]_{dce} - \frac{1}{4} g^{ab} W[\nabla]_{cedf} W[\nabla]^{cdef},$   
 $W[\nabla]^{acde} W[\nabla]_c^b W[\nabla]_{cde} - W[\nabla]^{acde} W[\nabla]_c^b W[\nabla]_{dce} - \frac{1}{4} g^{ab} W[\nabla]_{cdef} W[\nabla]^{cdef} +$   
 $\frac{1}{4} g^{ab} W[\nabla]_{cedf} W[\nabla]^{cdef}, W[\nabla]^{acde} W[\nabla]_c^b W[\nabla]_{cde} - 2 W[\nabla]^{acde} W[\nabla]_c^b W[\nabla]_{dce} -$   
 $\left. \frac{1}{4} g^{ab} W[\nabla]_{cdef} W[\nabla]^{cdef} + \frac{1}{2} g^{ab} W[\nabla]_{cedf} W[\nabla]^{cdef} \right\}$

These expressions are identically zero. Let's make rules for them:

**eom0ddisSol =**  
**First@SolveTensors[eom0ddis == 0, UseSymmetries -> False, MetricOn -> None]**

Solve::svars : Equations may not give solutions for all "solve" variables. >>

$\left\{ \text{HoldPattern}\left[ W[\nabla]_{\underline{acde}} W[\nabla]_{\underline{cde}}^b \right] \Rightarrow \right.$   
 $\text{Module}\left[ \{f, g, h, i\}, \frac{1}{4} g^{ab} W[\nabla]_{fghi} W[\nabla]^{fghi} \right],$   
 $\text{HoldPattern}\left[ W[\nabla]_{\underline{acde}} W[\nabla]_{\underline{dce}}^b \right] \Rightarrow$   
 $\left. \text{Module}\left[ \{f, g, h, i\}, \frac{1}{4} g^{ab} W[\nabla]_{fghi} W[\nabla]^{fghi} \right] \right\}$

Upon enforcing these rules, we see that the Weyl squared terms drop out, and we obtain exactly the Bach tensor:

**eom0 = eom0 /. eom0ddisSol // CollectTensors // SymmetrizeCovDs // RiemannToWeyl // ToCanonical**

$-2 R[\nabla]^{cd} W[\nabla]_c^a W[\nabla]_d^b - 4 (\nabla_{(cd} W[\nabla]^{acbd})$

Save it.

```
TensorPut[eom0]
```

```
eom0.m
```

Re-enable the definitions that make everything linear in Riemann tensor and remove the curvature relations.

```
SetLinearRiemann[];
```

```
ClearCurvatureRelations[CD];
```

```
Rules {17, 18} have been removed as DownValues for RicciCD.
```

```
Rules {1, 2, 3, 4, 5, 6, 7, 8, 9, 10, <<6>>} have been removed as UpValues for RicciCD.
```

```
Rules {1, 2, 3, 4, 5, 6, 7, 8, 9, 10, <<4>>}  
have been removed as DownValues for RiemannCD.
```

```
Rules {1, 2, 3, 4, 5, 6, 7, 8, 9, 10, <<14>>}  
have been removed as DownValues for SymRiemannCD.
```

## 3 Spin-3 action and equations of motion

### 3.0 Description

In this section we make an Ansatz for the quadratic spin-3 action and derive its equations of motion.

#### 3.1 Action

All possible terms including zero or one Riemann tensor are these:

```
actionterms = IndexFree@{  
  (* No curvature tensors. *)  
  phi CD@CD@CD@CD@CD@CD@phi,  
  (* One curvature tensor. *)  
  phi RiemannCD CD@CD@CD@CD@phi,  
  phi CD@RiemannCD CD@CD@CD@CD@phi,  
  phi CD@CD@RiemannCD CD@CD@CD@phi,  
  phi CD@CD@CD@RiemannCD CD@CD@phi,  
  phi CD@CD@CD@CD@RiemannCD phi  
}
```

$$\{\varphi \nabla \nabla \nabla \nabla \nabla \varphi, R[\nabla] \varphi \nabla \nabla \nabla \nabla \varphi, \varphi \nabla R[\nabla] \nabla \nabla \nabla \varphi, \\ \varphi \nabla \nabla R[\nabla] \nabla \nabla \varphi, \varphi \nabla \varphi \nabla \nabla \nabla R[\nabla], \varphi^2 \nabla \nabla \nabla \nabla R[\nabla]\}$$

Find all contractions of terms in the action.

```
actioncontractions = MapTimed[  
  AllContractions[#, Verbose → True] &,  
  actionterms  
];  
Length /@ actioncontractions  
Total[%]  
{4, 26, 68, 97, 68, 19}  
282
```

Make an Ansatz for the action.

```
actionAnsatz = MakeAnsatz[Flatten@actioncontractions, ConstantPrefix → "C"];
```

We know from the AdS analysis that the box cubed term is present. So without loss of generality,

we can fix its coefficient to be 1/2.

```
actionAnsatz /. RiemannCD[___] -> 0

C1  $\varphi^{abc} (\nabla_{(abc} \nabla_{def)} \varphi^{def}) + C2 \varphi^{abc} (\nabla_{(bcde} \nabla_{f)} \varphi_a^{de}) +$ 
   $C3 \varphi^{abc} (\nabla_{(cd} \nabla_{e} \nabla_{f)} \varphi_{ab}^d) + C4 \varphi^{abc} (\nabla^{(d} \nabla_{e} \nabla_{f)} \varphi_{abc})$ 

actionAnsatz = actionAnsatz /. C4 -> 1/2;
actionAnsatz /. RiemannCD[___] -> 0

C1  $\varphi^{abc} (\nabla_{(abc} \nabla_{def)} \varphi^{def}) + C2 \varphi^{abc} (\nabla_{(bcde} \nabla_{f)} \varphi_a^{de}) +$ 
   $C3 \varphi^{abc} (\nabla_{(cd} \nabla_{e} \nabla_{f)} \varphi_{ab}^d) + \frac{1}{2} \varphi^{abc} (\nabla^{(d} \nabla_{e} \nabla_{f)} \varphi_{abc})$ 
```

Save it.

```
TensorPut[actionAnsatz]
actionAnsatz.m

TensorGet[actionAnsatz]
actionAnsatz.m
```

## 3.2 Equations of motion

Compute the equations of motion. Note that we contract again with a generic symmetric rank 3 traceless tensor (T3TF) to reduce the number of terms.

```
eomAnsatz = CollectTensors@MapTimed[
  CollectTensors@SymmetrizeCovDs@
    CollectTensors[T3TF[-a, -b, -c] VarD[phi[-a, -b, -c], CD][#]] &,
  actionAnsatz
];

eomAnsatz // Length
eomAnsatz // TermsOf
289

{Ttf  $\nabla \nabla \nabla R[\nabla] \nabla \nabla \varphi$ , Ttf  $\nabla R[\nabla] \nabla \nabla \nabla \varphi$ , Ttf  $\nabla \varphi \nabla \nabla \nabla R[\nabla]$ ,
   $R[\nabla] \nabla \nabla \nabla \varphi$ , Ttf  $\varphi \nabla \nabla \nabla \nabla R[\nabla]$ , Ttf  $\nabla \nabla \nabla \nabla \nabla \varphi$ }

TensorPut[eomAnsatz]
eomAnsatz.m
```

## 4 Gauge invariance

### 4.0 Description

In this section we fix the Ansatz of the previous section by demanding invariance of the action under the gauge transformations

$$\begin{aligned} \delta_\xi \varphi_{abc} &= P \nabla_{(a} \xi_{bc)}, \\ \delta_\xi g_{ab} &= (\varphi \nabla \nabla \nabla \xi)_{ab} + \dots, \end{aligned} \tag{4}$$

### 4.1 Setup

First make a rule that sends the auxiliary tensor in the equations of motion of the spin 3 field to the

gauge variation of the spin 3 field.

```
t3toδphiRule = MakeRule@Evaluate@{
  T3TF[-a, -b, -c],
  CollectTensors[TFprojector CD[-d]@xi[-e, -f]]
}

{HoldPattern[Ttfabc] := Module[{d},  $\frac{1}{3} (\nabla^a \xi^{bc}) + \frac{1}{3} (\nabla^b \xi^{ac}) +$ 
 $\frac{1}{3} (\nabla^c \xi^{ab}) - \frac{1}{9} g^{cb} (\nabla_d \xi^{ad}) - \frac{1}{9} g^{ca} (\nabla_d \xi^{bd}) - \frac{1}{9} g^{ba} (\nabla_d \xi^{cd})$ ]}]
```

Also make an Ansatz for the gauge transformation of the metric under spin 3 transformations.

```
δgAnsatz = MakeContractionAnsatz[IndexFree@{
  phi CD@CD@CD@xi,
  CD@phi CD@CD@xi,
  CD@CD@phi CD@xi,
  CD@CD@CD@phi xi
},
{-a, -b}, Symmetric[{-a, -b}],
ConstantPrefix → "A",
Verbose → True
];
δgAnsatz // Length
66
```

## 4.2 Total variation

```
TensorGet[eomAnsatz]
```

```
eomAnsatz.m
```

```
TensorGet[eom0]
```

```
eom0.m
```

```
eom0linear = eom0 // ToRiemann // RicciToRiemann // ProjectRiemanns
```

$$-\frac{4}{3} (\nabla_{(cd)} R[\nabla]^{acbd}) + \frac{1}{3} g^{ab} (\nabla_{(de)} R[\nabla]^{cd}{}^e{}_c) -$$

$$\frac{2}{3} (\nabla^{(d}{}_{cd} R[\nabla]^{ac}{}_{b)} + \frac{1}{6} g^{ab} (\nabla^{(e}{}_{e)} R[\nabla]^{cd}{}_{cd})$$

```
TensorPut[eom0linear]
```

```
eom0linear.m
```

The gauge variation of the Weyl action under spin 3 transformations is:

```
δS0 = eom0linear * ReplaceDummies[δgAnsatz] // CollectTensors;
```

The gauge variations of the spin 3 part of the action is:

```
δS2 = eomAnsatz /. t3toδphiRule // CollectTensors;
```

The total gauge variation is then:

```
δtotal = δS0 + δS2 // CollectTensors[#, Verbose → True] &;
```

```

** Collecting tensors in expression of length 930 and head Plus.
** Expanded to 930 tensorial terms in 0.68s.
** Found 10 dummies, {a, b, c, d, e, f, g, l$23816, l$26187, l$26188} in 0.82s.
** Replaced dummies in 1.77s.
** Applied TensorWrapper in 0.34s.
** Found 886 TensorWrappers in 0.01s.
** Canonicalized 886 TensorWrappers in 13.05s.
** Replaced TensorWrappers in 0.65s.
** Collected TensorWrappers in 1.72s.
** Simplified coefficient of each term in 0.32s.

```

```
 $\delta$ total // Length
```

```
 $\delta$ total // ConstantSymbolsOf
```

```
 $\delta$ total // TermsOf
```

```
886
```

```

{A1, A10, A11, A12, A13, A14, A15, A16, A17, A18, A2, A20, A21, A22, A23, A24, A25, A26, A27,
A28, A3, A30, A31, A32, A33, A36, A37, A38, A39, A4, A41, A45, A46, A47, A48, A49, A5,
A50, A51, A52, A53, A54, A55, A56, A57, A58, A6, A61, A62, A63, A64, A7, A8, A9, C1,
C10, C100, C101, C102, C103, C104, C105, C106, C107, C108, C109, C11, C110, C111, C112,
C113, C114, C115, C116, C117, C118, C119, C12, C120, C121, C122, C123, C124, C125, C126,
C127, C128, C129, C13, C130, C131, C132, C133, C134, C135, C136, C137, C138, C139, C14,
C140, C141, C142, C143, C144, C145, C146, C147, C148, C149, C15, C150, C151, C152, C153,
C154, C155, C156, C157, C158, C159, C16, C160, C161, C162, C163, C164, C165, C166, C167,
C168, C169, C17, C170, C171, C172, C173, C174, C175, C176, C177, C178, C179, C18, C180,
C181, C182, C183, C184, C185, C186, C187, C188, C189, C19, C190, C191, C192, C193, C194,
C195, C196, C197, C198, C199, C2, C20, C200, C201, C202, C203, C204, C205, C206, C207,
C208, C209, C21, C210, C211, C212, C213, C214, C215, C216, C217, C218, C219, C22, C220,
C221, C222, C223, C224, C225, C226, C227, C228, C229, C23, C230, C231, C232, C233, C234,
C235, C236, C237, C238, C239, C24, C240, C241, C242, C243, C244, C245, C246, C247, C248,
C249, C25, C250, C251, C252, C253, C254, C255, C256, C257, C258, C259, C26, C260, C261,
C262, C263, C264, C265, C266, C267, C268, C269, C27, C270, C271, C272, C273, C274, C275,
C276, C277, C278, C279, C28, C280, C281, C282, C29, C3, C30, C31, C32, C33, C34, C35,
C36, C37, C38, C39, C40, C41, C42, C43, C44, C45, C46, C47, C48, C49, C5, C50, C51,
C52, C53, C54, C55, C56, C57, C58, C59, C6, C60, C61, C62, C63, C64, C65, C66, C67,
C68, C69, C7, C70, C71, C72, C73, C74, C75, C76, C77, C78, C79, C8, C80, C81, C82, C83,
C84, C85, C86, C87, C88, C89, C9, C90, C91, C92, C93, C94, C95, C96, C97, C98, C99}

```

```

{ $\nabla \xi \nabla \nabla R[\nabla] \nabla \nabla \varphi$ ,  $\nabla \varphi \nabla \nabla R[\nabla] \nabla \nabla \xi$ ,  $\nabla R[\nabla] \nabla \xi \nabla \nabla \nabla \varphi$ ,  $\xi \nabla \nabla R[\nabla] \nabla \nabla \nabla \varphi$ ,  $\nabla \xi \nabla \varphi \nabla \nabla \nabla R[\nabla]$ ,
 $\varphi \nabla \nabla R[\nabla] \nabla \nabla \nabla \xi$ ,  $R[\nabla] \nabla \xi \nabla \nabla \nabla \nabla \varphi$ ,  $\varphi \nabla \xi \nabla \nabla \nabla \nabla R[\nabla]$ ,  $\nabla \xi \nabla \nabla \nabla \nabla \nabla \varphi$ }

```

```
TensorPut[ $\delta$ total]
```

```
 $\delta$ total.m
```

Integrate by parts in order to remove all derivatives on the gauge parameter:

```

 $\delta$ totalPI = CollectTensors@MapTimedTensors[
  CollectTensors@
    SymmetrizeCovDs@CollectTensors[xi[-a, -b] VarD[xi[-a, -b], CD][#]] &,
   $\delta$ total
];

```

```

δtotalPI // TermsOf
δtotalPI // Length

{ξ ∇ ∇ ∇ R[∇] ∇ ∇ ∇ φ, ξ ∇ ∇ φ ∇ ∇ ∇ R[∇], ξ ∇ R[∇] ∇ ∇ ∇ ∇ φ,
  ξ ∇ φ ∇ ∇ ∇ ∇ R[∇], R[∇] ξ ∇ ∇ ∇ ∇ ∇ φ, ξ φ ∇ ∇ ∇ ∇ ∇ R[∇], ξ ∇ ∇ ∇ ∇ ∇ ∇ ∇ φ}

437

TensorPut[δtotalPI]
δtotalPI.m

```

### 4.3 DDIs

We also need to compute any Dimensional Dependent Identities (DDIs) that may appear in the total gauge variation before we can impose it to be zero.

First, construct the DDIs for each of the different kind of terms that appear in the total variation:

```

δtotalPiDDIs = ProjectRiemanns@MapTimed[
  ConstructDDIs[#, Verbose → True] &,
  TermsOf@δtotalPI
];

** DefTensor: Defining basic dimensional dependent identity
BasicDDICD4[-a, -b, -c, -d, -e, -f, -g, -h, -i, -j].

Length /@ δtotalPiDDIs
Total[%]

{25, 25, 8, 8, 1, 1, 0}

68

```

Next, flatten out the DDIs, and remove any overall factors and zeros:

```

δtotalPiDDIs = xAct`xTras`Private`DeleteDuplicateFactors@Flatten@δtotalPiDDIs
δtotalPiDDIs // Length

6

```

Save:

```

TensorPut[δtotalPiDDIs]
δtotalPiDDIs.m

```

### 4.4 Invariance

```

TensorGet[δtotalPiDDIs]
δtotalPiDDIs.m

TensorGet[δtotalPI]
δtotalPI.m

```



**$\delta$ totalPI // ConstantSymbolsOf**

```
{A1, A10, A11, A12, A13, A14, A15, A16, A17, A18, A2, A20, A21, A22, A23, A24, A25, A26, A27,
A28, A3, A30, A31, A32, A33, A36, A37, A38, A39, A4, A41, A45, A46, A47, A48, A49, A5,
A50, A51, A52, A53, A54, A55, A56, A57, A58, A6, A61, A62, A63, A64, A7, A8, A9, C1,
C10, C100, C101, C102, C103, C104, C105, C106, C107, C108, C109, C11, C110, C111, C112,
C113, C114, C115, C116, C117, C118, C119, C12, C120, C121, C122, C123, C124, C125, C126,
C127, C128, C129, C13, C130, C131, C132, C133, C134, C135, C136, C137, C138, C139, C14,
C140, C141, C142, C143, C144, C145, C146, C147, C148, C149, C15, C150, C151, C152, C153,
C154, C155, C156, C157, C158, C159, C16, C160, C161, C162, C163, C164, C165, C166, C167,
C168, C169, C17, C170, C171, C172, C173, C174, C175, C176, C177, C178, C179, C18, C180,
C181, C182, C183, C184, C185, C186, C187, C188, C189, C19, C190, C191, C192, C193, C194,
C195, C196, C197, C198, C199, C2, C20, C200, C201, C202, C203, C204, C205, C206, C207,
C208, C209, C21, C210, C211, C212, C213, C214, C215, C216, C217, C218, C219, C22, C220,
C221, C222, C223, C224, C225, C226, C227, C228, C229, C23, C230, C231, C232, C233, C234,
C235, C236, C237, C238, C239, C24, C240, C241, C242, C243, C244, C245, C246, C247, C248,
C249, C25, C250, C251, C252, C253, C254, C255, C256, C257, C258, C259, C26, C260, C261,
C262, C263, C264, C265, C266, C267, C268, C269, C27, C270, C271, C272, C273, C274, C275,
C276, C277, C278, C279, C28, C280, C281, C282, C29, C3, C30, C31, C32, C33, C34, C35,
C36, C37, C38, C39, C40, C41, C42, C43, C44, C45, C46, C47, C48, C49, C5, C50, C51,
C52, C53, C54, C55, C56, C57, C58, C59, C6, C60, C61, C62, C63, C64, C65, C66, C67,
C68, C69, C7, C70, C71, C72, C73, C74, C75, C76, C77, C78, C79, C8, C80, C81, C82, C83,
C84, C85, C86, C87, C88, C89, C9, C90, C91, C92, C93, C94, C95, C96, C97, C98, C99}
```

**$\delta$ totalZero =**

**ProjectRiemanns[ $\delta$ totalPI + MakeAnsatz[ $\delta$ totalPiDDIs, ConstantPrefix → "E"]];**

**$\delta$ totalZero // Length**

**$\delta$ totalZero // ConstantSymbolsOf**

437

```
{A1, A10, A11, A12, A13, A14, A15, A16, A17, A18, A2, A20, A21, A22, A23, A24, A25, A26, A27,
A28, A3, A30, A31, A32, A33, A36, A37, A38, A39, A4, A41, A45, A46, A47, A48, A49, A5,
A50, A51, A52, A53, A54, A55, A56, A57, A58, A6, A61, A62, A63, A64, A7, A8, A9, C1, C10,
C100, C101, C102, C103, C104, C105, C106, C107, C108, C109, C11, C110, C111, C112, C113,
C114, C115, C116, C117, C118, C119, C12, C120, C121, C122, C123, C124, C125, C126, C127,
C128, C129, C13, C130, C131, C132, C133, C134, C135, C136, C137, C138, C139, C14, C140,
C141, C142, C143, C144, C145, C146, C147, C148, C149, C15, C150, C151, C152, C153, C154,
C155, C156, C157, C158, C159, C16, C160, C161, C162, C163, C164, C165, C166, C167, C168,
C169, C17, C170, C171, C172, C173, C174, C175, C176, C177, C178, C179, C18, C180, C181,
C182, C183, C184, C185, C186, C187, C188, C189, C19, C190, C191, C192, C193, C194, C195,
C196, C197, C198, C199, C2, C20, C200, C201, C202, C203, C204, C205, C206, C207, C208,
C209, C21, C210, C211, C212, C213, C214, C215, C216, C217, C218, C219, C22, C220, C221,
C222, C223, C224, C225, C226, C227, C228, C229, C23, C230, C231, C232, C233, C234, C235,
C236, C237, C238, C239, C24, C240, C241, C242, C243, C244, C245, C246, C247, C248, C249,
C25, C250, C251, C252, C253, C254, C255, C256, C257, C258, C259, C26, C260, C261, C262,
C263, C264, C265, C266, C267, C268, C269, C27, C270, C271, C272, C273, C274, C275, C276,
C277, C278, C279, C28, C280, C281, C282, C29, C3, C30, C31, C32, C33, C34, C35, C36, C37,
C38, C39, C40, C41, C42, C43, C44, C45, C46, C47, C48, C49, C5, C50, C51, C52, C53, C54,
C55, C56, C57, C58, C59, C6, C60, C61, C62, C63, C64, C65, C66, C67, C68, C69, C7, C70,
C71, C72, C73, C74, C75, C76, C77, C78, C79, C8, C80, C81, C82, C83, C84, C85, C86, C87,
C88, C89, C9, C90, C91, C92, C93, C94, C95, C96, C97, C98, C99, E1, E2, E3, E4, E5, E6}
```

**TensorPut[ $\delta$ totalZero]**

$\delta$ totalZero.m

**TensorGet[ $\delta$ totalZero]**

$\delta$ totalZero.m

There is exactly one solution (which makes sense, because the equation is linear in the variables we solve for):

```
SolveConstants [ $\delta$ totalZero == 0];
% // Length
gaugesol = %[[1]];
```

Solve::svars : Equations may not give solutions for all "solve" variables. >>

1

There are however no solutions if we don't use the DDIs or if we don't use the compensating gauge variation of the metric.

```
dontsolveforvars = Complement [
  ConstantSymbolsOf [ $\delta$ totalZero],
  ConstantSymbolsOf [eomAnsatz]
]
{A1, A10, A11, A12, A13, A14, A15, A16, A17, A18, A2, A20, A21, A22, A23, A24, A25, A26, A27,
A28, A3, A30, A31, A32, A33, A36, A37, A38, A39, A4, A41, A45, A46, A47, A48, A49, A5, A50, A51,
A52, A53, A54, A55, A56, A57, A58, A6, A61, A62, A63, A64, A7, A8, A9, E1, E2, E3, E4, E5, E6}
```

Turn everything off:

```
SolveConstants [ $\delta$ totalZero == 0, ! dontsolveforvars];
% // Length
0
```

Turn only the gauge variation of the metric off:

```
SolveConstants [ $\delta$ totalZero == 0, ! (dontsolveforvars[[1 ;; -7]])];
% // Length
0
```

Turn only the DDIs off:

```
SolveConstants [ $\delta$ totalZero == 0, ! (dontsolveforvars[[-6 ;; -1]])];
% // Length
$Aborted
0
```

```
action = actionAnsatz /. gaugesol;
```

```
eom = eomAnsatz /. gaugesol;
```

```
 $\delta$ g =  $\delta$ gAnsatz /. gaugesol;
```

```
eom /. RiemannCD[__] → 0
```

$$-\frac{2}{5} \text{Ttf}^{abc} \left( \nabla_{(abcdef)} \varphi^{def} \right) + \frac{12}{5} \text{Ttf}^{abc} \left( \nabla_{(bcde}{}^f{}_{f)} \varphi_a{}^{de} \right) -$$

$$3 \text{Ttf}^{abc} \left( \nabla_{(cd}{}^e{}_{ef)} \varphi_{ab}{}^d \right) + \text{Ttf}^{abc} \left( \nabla^{(d}{}^e{}_{ef)} \varphi_{abc} \right)$$

```
eom // ConstantSymbolsOf
```

```
{A1, A10, A11, A13, A14, A15, A16, A17, A18, A20, A26, A36, A4, A46, A50, C10, C100,  
C101, C102, C103, C104, C105, C106, C107, C108, C109, C11, C110, C111, C112, C113, C114,  
C115, C116, C117, C118, C119, C120, C121, C122, C123, C124, C125, C126, C127, C128,  
C129, C130, C131, C132, C133, C134, C135, C136, C137, C138, C139, C14, C140, C141, C142,  
C143, C144, C145, C146, C147, C148, C149, C15, C150, C151, C152, C153, C154, C155, C156,  
C157, C158, C159, C16, C160, C161, C162, C163, C164, C165, C166, C167, C168, C169, C17,  
C170, C171, C172, C173, C174, C175, C176, C177, C178, C179, C18, C180, C181, C182, C184,  
C185, C186, C187, C188, C19, C190, C192, C193, C197, C198, C199, C200, C201, C202, C203,  
C204, C205, C206, C207, C208, C209, C211, C212, C213, C214, C215, C216, C217, C218,  
C219, C22, C220, C221, C222, C223, C224, C225, C226, C227, C228, C229, C230, C231,  
C232, C233, C235, C236, C237, C238, C239, C240, C241, C242, C243, C244, C245, C247,  
C249, C251, C253, C255, C256, C258, C259, C260, C263, C264, C265, C267, C268, C269,  
C270, C271, C272, C276, C277, C279, C31, C32, C35, C36, C38, C39, C41, C42, C43, C46,  
C47, C49, C52, C56, C60, C63, C65, C69, C71, C73, C78, C83, C84, C85, C87, C91, C95}
```

```
TensorPut[action]
```

```
action.m
```

```
TensorPut[eom]
```

```
eom.m
```

```
TensorPut[gaugesol]
```

```
gaugesol.m
```

```
TensorPut[δg]
```

```
δg.m
```

## 5 Uniqueness

### 5.0 Description

In this section we show that the gauge invariant equations of motion that we obtained in the previous section are in fact unique, modulo field redefinitions and DDIs.

#### 5.1 EOM DDIs

Here we construct all DDIs that are relevant for the equations of motion.

```
eomDDIs = ProjectRiemanns@MapTimed[  
  ConstructDDIs[#, Verbose → True] &,  
  TermsOf@eomAnsatz  
];
```

```
Length/@eomDDIs  
Total[%]  
{22, 10, 10, 2, 2, 0}
```

```
46
```

Flatten out the DDIs, remove the overall factors and duplicates:

```
eomDDIs = xAct`xTras`Private`DeleteDuplicateFactors@Flatten@eomDDIs;  
eomDDIs // Length
```

```
7
```

Save:

```
TensorPut[eomDDIs]
eomDDIs.m
```

## 5.2 Field redefinitions

In this section we deduce what contributions to the spin-3 action and equations of motions can arise due to field redefinitions of the metric.

These contributions are proportional to the equations of motion of the metric, which reads in its linearized form:

```
TensorGet[eom0linear]
eom0linear.m
```

All the possible field redefinitions of the metric are:

```
metricredefs = MakeContractionAnsatz[IndexFree@{phi CD@CD@phi, CD@phi CD@phi},
  {-a, -b}, Symmetric[{-a, -b}], Verbose -> True, ConstantPrefix -> "D"]
```

$$\begin{aligned}
& D_1 (\nabla_a \varphi^{cde}) (\nabla_b \varphi_{cde}) + D_2 (\nabla_c \varphi_a^{cd}) (\nabla_e \varphi_{bd}^e) + \\
& D_3 (\nabla^d \varphi_{ab}^c) (\nabla_e \varphi_{cd}^e) + D_4 ((\nabla_a \varphi_b^{cd}) (\nabla_e \varphi_{cd}^e) + (\nabla_b \varphi_a^{cd}) (\nabla_e \varphi_{cd}^e)) + \\
& D_5 (\nabla_d \varphi_{bce}) (\nabla^e \varphi_a^{cd}) + D_6 (\nabla_e \varphi_{bcd}) (\nabla^e \varphi_a^{cd}) + \\
& D_7 ((\nabla_b \varphi_{cde}) (\nabla^e \varphi_a^{cd}) + (\nabla_a \varphi_{cde}) (\nabla^e \varphi_b^{cd})) + D_8 g_{ab} (\nabla_c \varphi^{cde}) (\nabla_f \varphi_{de}^f) + \\
& D_9 g_{ab} (\nabla_e \varphi_{cdf}) (\nabla^f \varphi^{cde}) + D_{10} g_{ab} (\nabla_f \varphi_{cde}) (\nabla^f \varphi^{cde}) + \\
& D_{11} \varphi^{cde} (\nabla_{(ab)} \varphi_{cde}) + D_{12} (\varphi^{cde} (\nabla_{(ae)} \varphi_{bcd}) + \varphi^{cde} (\nabla_{(be)} \varphi_{acd})) + \\
& D_{13} (\varphi_b^{cd} (\nabla_{(ae)} \varphi_{cd}^e) + \varphi_a^{cd} (\nabla_{(be)} \varphi_{cd}^e)) + \\
& D_{14} \varphi^{cde} (\nabla_{(de)} \varphi_{abc}) + D_{15} (\varphi_b^{cd} (\nabla_{(de)} \varphi_{ac}^e) + \varphi_a^{cd} (\nabla_{(de)} \varphi_{bc}^e)) + \\
& D_{16} \varphi_{ab}^c (\nabla_{(de)} \varphi_c^{de}) + D_{17} g_{ab} \varphi^{cde} (\nabla_{(ef)} \varphi_{cd}^f) + \\
& D_{18} (\varphi_b^{cd} (\nabla^{(e)} \varphi_{acd}) + \varphi_a^{cd} (\nabla^{(e)} \varphi_{bcd})) + D_{19} g_{ab} \varphi^{cde} (\nabla^{(f)} \varphi_{cde})
\end{aligned}$$

The contributions to the spin-3 actions are then:

```
S2redef = eom0linear * ReplaceDummies@metricredefs // CollectTensors
```

$$\begin{aligned}
& -\frac{4}{3} D_{16} \varphi^{abc} (\nabla_{(de)} \varphi_a^{de}) (\nabla_{(fg)} R[\nabla]_b^f c^g) - \frac{8}{3} D_{18} \varphi^{abc} (\nabla^{(e)} \varphi_{ab}^d) (\nabla_{(fg)} R[\nabla]_c^f d^g) - \\
& \frac{4}{3} D_2 (\nabla_a \varphi^{abc}) (\nabla_d \varphi_b^{de}) (\nabla_{(fg)} R[\nabla]_c^f e^g) - \frac{4}{3} D_5 (\nabla_b \varphi_{ad}^e) (\nabla^d \varphi^{abc}) (\nabla_{(fg)} R[\nabla]_c^f e^g) - \\
& \frac{4}{3} D_6 (\nabla_d \varphi_{ab}^e) (\nabla^d \varphi^{abc}) (\nabla_{(fg)} R[\nabla]_c^f e^g) - \frac{8}{3} D_7 (\nabla^d \varphi^{abc}) (\nabla^e \varphi_{abd}) (\nabla_{(fg)} R[\nabla]_c^f e^g) - \\
& \frac{8}{3} D_{15} \varphi^{abc} (\nabla_{(bd)} \varphi_a^{de}) (\nabla_{(fg)} R[\nabla]_c^f e^g) - \frac{8}{3} D_{13} \varphi^{abc} (\nabla_{(d)}^e \varphi_{ab}^d) (\nabla_{(fg)} R[\nabla]_c^f e^g) - \\
& \frac{4}{3} D_3 (\nabla_a \varphi^{abc}) (\nabla_c \varphi_b^{de}) (\nabla_{(fg)} R[\nabla]_d^f e^g) - \frac{4}{3} D_1 (\nabla^d \varphi^{abc}) (\nabla^e \varphi_{abc}) (\nabla_{(fg)} R[\nabla]_d^f e^g) - \\
& \frac{8}{3} D_4 (\nabla_a \varphi^{abc}) (\nabla^e \varphi_{bc}^d) (\nabla_{(fg)} R[\nabla]_d^f e^g) - \frac{4}{3} D_{14} \varphi^{abc} (\nabla_{(bc)} \varphi_a^{de}) (\nabla_{(fg)} R[\nabla]_d^f e^g) - \\
& \frac{8}{3} D_{12} \varphi^{abc} (\nabla_{(c)}^e \varphi_{ab}^d) (\nabla_{(fg)} R[\nabla]_d^f e^g) - \frac{4}{3} D_{11} \varphi^{abc} (\nabla^{(de)} \varphi_{abc}) (\nabla_{(fg)} R[\nabla]_d^f e^g) + \\
& \left( \frac{D_2}{3} + \frac{2 D_4}{3} \right) (\nabla_a \varphi^{abc}) (\nabla_d \varphi_{bc}^d) (\nabla_{(fg)} R[\nabla]^{ef} e^g) + \\
& \left( \frac{D_5}{3} + \frac{2 D_7}{3} \right) (\nabla_c \varphi_{abd}) (\nabla^d \varphi^{abc}) (\nabla_{(fg)} R[\nabla]^{ef} e^g) + \\
& \left( \frac{D_1}{3} + \frac{D_6}{3} \right) (\nabla_d \varphi_{abc}) (\nabla^d \varphi^{abc}) (\nabla_{(fg)} R[\nabla]^{ef} e^g) + \\
& \left( \frac{2 D_{12}}{3} + \frac{2 D_{13}}{3} + \frac{2 D_{15}}{3} \right) \varphi^{abc} (\nabla_{(cd)} \varphi_{ab}^d) (\nabla_{(fg)} R[\nabla]^{ef} e^g) + \\
& \left( \frac{D_{11}}{3} + \frac{2 D_{18}}{3} \right) \varphi^{abc} (\nabla^{(d)} \varphi_{abc}) (\nabla_{(fg)} R[\nabla]^{ef} e^g) - \\
& \frac{2}{3} D_{16} \varphi^{abc} (\nabla_{(de)} \varphi_a^{de}) (\nabla^{(g)} R[\nabla]_b^f c^f) - \frac{4}{3} D_{18} \varphi^{abc} (\nabla^{(e)} \varphi_{ab}^d) (\nabla^{(g)} R[\nabla]_c^f d^f) - \\
& \frac{2}{3} D_2 (\nabla_a \varphi^{abc}) (\nabla_d \varphi_b^{de}) (\nabla^{(g)} R[\nabla]_c^f e^f) - \frac{2}{3} D_5 (\nabla_b \varphi_{ad}^e) (\nabla^d \varphi^{abc}) (\nabla^{(g)} R[\nabla]_c^f e^f) - \\
& \frac{2}{3} D_6 (\nabla_d \varphi_{ab}^e) (\nabla^d \varphi^{abc}) (\nabla^{(g)} R[\nabla]_c^f e^f) - \frac{4}{3} D_7 (\nabla^d \varphi^{abc}) (\nabla^e \varphi_{abd}) (\nabla^{(g)} R[\nabla]_c^f e^f) - \\
& \frac{4}{3} D_{15} \varphi^{abc} (\nabla_{(bd)} \varphi_a^{de}) (\nabla^{(g)} R[\nabla]_c^f e^f) - \frac{4}{3} D_{13} \varphi^{abc} (\nabla_{(d)}^e \varphi_{ab}^d) (\nabla^{(g)} R[\nabla]_c^f e^f) - \\
& \frac{2}{3} D_3 (\nabla_a \varphi^{abc}) (\nabla_c \varphi_b^{de}) (\nabla^{(g)} R[\nabla]_d^f e^f) - \frac{2}{3} D_1 (\nabla^d \varphi^{abc}) (\nabla^e \varphi_{abc}) (\nabla^{(g)} R[\nabla]_d^f e^f) - \\
& \frac{4}{3} D_4 (\nabla_a \varphi^{abc}) (\nabla^e \varphi_{bc}^d) (\nabla^{(g)} R[\nabla]_d^f e^f) - \frac{2}{3} D_{14} \varphi^{abc} (\nabla_{(bc)} \varphi_a^{de}) (\nabla^{(g)} R[\nabla]_d^f e^f) - \\
& \frac{4}{3} D_{12} \varphi^{abc} (\nabla_{(c)}^e \varphi_{ab}^d) (\nabla^{(g)} R[\nabla]_d^f e^f) - \frac{2}{3} D_{11} \varphi^{abc} (\nabla^{(de)} \varphi_{abc}) (\nabla^{(g)} R[\nabla]_d^f e^f) + \\
& \left( \frac{D_2}{6} + \frac{D_4}{3} \right) (\nabla_a \varphi^{abc}) (\nabla_d \varphi_{bc}^d) (\nabla^{(g)} R[\nabla]^{ef} e^f) + \\
& \left( \frac{D_5}{6} + \frac{D_7}{3} \right) (\nabla_c \varphi_{abd}) (\nabla^d \varphi^{abc}) (\nabla^{(g)} R[\nabla]^{ef} e^f) + \\
& \left( \frac{D_1}{6} + \frac{D_6}{6} \right) (\nabla_d \varphi_{abc}) (\nabla^d \varphi^{abc}) (\nabla^{(g)} R[\nabla]^{ef} e^f) + \\
& \left( \frac{D_{12}}{3} + \frac{D_{13}}{3} + \frac{D_{15}}{3} \right) \varphi^{abc} (\nabla_{(cd)} \varphi_{ab}^d) (\nabla^{(g)} R[\nabla]^{ef} e^f) + \\
& \left( \frac{D_{11}}{6} + \frac{D_{18}}{3} \right) \varphi^{abc} (\nabla^{(d)} \varphi_{abc}) (\nabla^{(g)} R[\nabla]^{ef} e^f)
\end{aligned}$$

The contributions to the equations of motion are then:

```
eomredef = CollectTensors@MapTimedTensors[
  CollectTensors@SymmetrizeCovDs@
    CollectTensors[T3TF[-a, -b, -c] VarD[phi[-a, -b, -c], CD][#]] &,
  S2redef
];

eomredef = eomredef // ProjectRiemanns;

TensorPut[eomredef]
eomredef.m
```

### 5.3 Eliminating total derivatives

In this section we derive which constants in the ‘total equations of motion’ (i.e. the one derived from the action, plus DDIS, plus field redefs) parameterize total derivatives.

```
TensorGet[eomDDIs]
eomDDIs.m
```

```
TensorGet[eom]
eom.m
```

The total equations of motion are:

```
ddisAnsatz = MakeAnsatz[eomDDIs, ConstantPrefix → "B"];

totaleom = ddisAnsatz + eom + eomredef // CollectTensors // ProjectRiemanns;

TensorPut[totaleom]
totaleom.m
```

Select the piece that depends on the unfixed constants:

```
unfixedeom = totaleom -
  (totaleom /. (# → 0 & /@ ConstantSymbolsOf[totaleom])) // CollectTensors;
```

Show that we can remove all unfixed constants in the equations of motion by tuning the DDIs and / or the field redefinitions:

```
SolveConstants[unfixedeom == 0, ConstantSymbolsOf[{ddisAnsatz, eomredef}]];
% // Length
```

Solve::svars : Equations may not give solutions for all "solve" variables. >>

1

And indeed we can. This means that the equations of motion are unique up to field redefinitions and DDIs.

## 6 Factorization

### 6.0 Description

In this section we show that the equations of motion do not factorize into 3 factors that each have 2 derivatives.

#### 6.1 Ansatz

Let's assume that the equations of motion factorize into  $O_1 \cdot O_2 \cdot O_3 \cdot \varphi$ , where

$(O_i)_{abc}^{def} \simeq (\nabla \nabla \delta \delta + R \delta)_{abc}^{def}$ . We don't need to consider traces of the higher spin field because they would have to cancel by themselves anyhow, so we can just focus our attention on the traceless part.

Find the most general  $O_i$  operator.

```
O1ansatz = ProjectRiemanns@MakeContractionAnsatz [  
  IndexFree@{ T3 CD@CD@phi, T3 RiemannCD phi},  
  ConstantPrefix -> "α",  
  Verbose -> True  
] /. α7 -> 1
```

$$\begin{aligned} & \alpha_1 \varphi^{abc} R[\nabla]_{de}^{de} T_{abc} + \alpha_2 \varphi^{abc} R[\nabla]_c^e{}_{de} T_{ab}^d + \\ & \alpha_3 \varphi^{abc} R[\nabla]_b^e{}_{ce} T_a^d + \alpha_4 \varphi^{abc} R[\nabla]_{bdce} T_a^{de} + \\ & \alpha_5 T^{abc} (\nabla_{(cd)} \varphi_{ab}^d) + \alpha_6 T_a^{ab} (\nabla_{(cd)} \varphi_b^{cd}) + T^{abc} (\nabla^{(d)}{}_{(d)} \varphi_{abc}) \end{aligned}$$

Construct the other two by just renaming the constant symbols:

```
αs = ConstantSymbolsOf [O1ansatz]  
βs = DefNiceConstantSymbol ["β", #] & /@ Range@Length [%] // Sort  
γs = DefNiceConstantSymbol ["γ", #] & /@ Range@Length [%] // Sort  
{α1, α2, α3, α4, α5, α6}  
  
{β1, β2, β3, β4, β5, β6}  
  
{γ1, γ2, γ3, γ4, γ5, γ6}
```

```
O2ansatz = O1ansatz /. Inner [Rule, αs, βs, List]
```

```
O3ansatz = O1ansatz /. Inner [Rule, αs, γs, List]
```

$$\begin{aligned} & \beta_1 \varphi^{abc} R[\nabla]_{de}^{de} T_{abc} + \beta_2 \varphi^{abc} R[\nabla]_c^e{}_{de} T_{ab}^d + \\ & \beta_3 \varphi^{abc} R[\nabla]_b^e{}_{ce} T_a^d + \beta_4 \varphi^{abc} R[\nabla]_{bdce} T_a^{de} + \\ & \beta_5 T^{abc} (\nabla_{(cd)} \varphi_{ab}^d) + \beta_6 T_a^{ab} (\nabla_{(cd)} \varphi_b^{cd}) + T^{abc} (\nabla^{(d)}{}_{(d)} \varphi_{abc}) \end{aligned}$$

$$\begin{aligned} & \gamma_1 \varphi^{abc} R[\nabla]_{de}^{de} T_{abc} + \gamma_2 \varphi^{abc} R[\nabla]_c^e{}_{de} T_{ab}^d + \\ & \gamma_3 \varphi^{abc} R[\nabla]_b^e{}_{ce} T_a^d + \gamma_4 \varphi^{abc} R[\nabla]_{bdce} T_a^{de} + \\ & \gamma_5 T^{abc} (\nabla_{(cd)} \varphi_{ab}^d) + \gamma_6 T_a^{ab} (\nabla_{(cd)} \varphi_b^{cd}) + T^{abc} (\nabla^{(d)}{}_{(d)} \varphi_{abc}) \end{aligned}$$

Chain the three operators by making a rule.

```

rule1 = MakeRule@
  Evaluate@{phi[-a, -b, -c], CollectTensors@VarD[T3[a, b, c]] [O1ansatz]}
rule2 = MakeRule@Evaluate@{phi[-a, -b, -c],
  CollectTensors@VarD[T3[a, b, c]] [O2ansatz]}

{HoldPattern[ $\varphi^{\underline{abc}}$ ] :=
  Module[{d, e, f},  $\frac{1}{3} \alpha_4 \varphi^{cde} R[\nabla]^a_d{}^b_e + \frac{1}{3} \alpha_4 \varphi^{bde} R[\nabla]^a_d{}^c_e + \frac{1}{3} \alpha_2 \varphi^{bcd} R[\nabla]^{ae}_{de} +$ 
 $\frac{1}{3} \alpha_4 \varphi^{ade} R[\nabla]^b_d{}^c_e + \frac{1}{3} \alpha_2 \varphi^{acd} R[\nabla]^{be}_{de} + \frac{1}{3} \alpha_2 \varphi^{abd} R[\nabla]^{ce}_{de} +$ 
 $\frac{1}{3} \alpha_3 g^{cb} \varphi^{ade} R[\nabla]^f_{def} + \frac{1}{3} \alpha_3 g^{ca} \varphi^{bde} R[\nabla]^f_{def} + \frac{1}{3} \alpha_3 g^{ba} \varphi^{cde} R[\nabla]^f_{def} +$ 
 $\alpha_1 \varphi^{abc} R[\nabla]^{de}_{de} + \frac{1}{3} \alpha_5 (\nabla^{(a}_d \varphi^{bcd)} + \frac{1}{3} \alpha_5 (\nabla^{(b}_d \varphi^{acd)} + \frac{1}{3} \alpha_5 (\nabla^{(c}_d \varphi^{abd)} +$ 
 $\frac{1}{3} \alpha_6 g^{cb} (\nabla_{(de)} \varphi^{ade}) + \frac{1}{3} \alpha_6 g^{ca} (\nabla_{(de)} \varphi^{bde}) + \frac{1}{3} \alpha_6 g^{ba} (\nabla_{(de)} \varphi^{cde}) + \nabla^{(d}_{de} \varphi^{abc}] ]$ 

{HoldPattern[ $\varphi^{\underline{abc}}$ ] :=
  Module[{d, e, f},  $\frac{1}{3} \beta_4 \varphi^{cde} R[\nabla]^a_d{}^b_e + \frac{1}{3} \beta_4 \varphi^{bde} R[\nabla]^a_d{}^c_e + \frac{1}{3} \beta_2 \varphi^{bcd} R[\nabla]^{ae}_{de} +$ 
 $\frac{1}{3} \beta_4 \varphi^{ade} R[\nabla]^b_d{}^c_e + \frac{1}{3} \beta_2 \varphi^{acd} R[\nabla]^{be}_{de} + \frac{1}{3} \beta_2 \varphi^{abd} R[\nabla]^{ce}_{de} +$ 
 $\frac{1}{3} \beta_3 g^{cb} \varphi^{ade} R[\nabla]^f_{def} + \frac{1}{3} \beta_3 g^{ca} \varphi^{bde} R[\nabla]^f_{def} + \frac{1}{3} \beta_3 g^{ba} \varphi^{cde} R[\nabla]^f_{def} +$ 
 $\beta_1 \varphi^{abc} R[\nabla]^{de}_{de} + \frac{1}{3} \beta_5 (\nabla^{(a}_d \varphi^{bcd)} + \frac{1}{3} \beta_5 (\nabla^{(b}_d \varphi^{acd)} + \frac{1}{3} \beta_5 (\nabla^{(c}_d \varphi^{abd)} +$ 
 $\frac{1}{3} \beta_6 g^{cb} (\nabla_{(de)} \varphi^{ade}) + \frac{1}{3} \beta_6 g^{ca} (\nabla_{(de)} \varphi^{bde}) + \frac{1}{3} \beta_6 g^{ba} (\nabla_{(de)} \varphi^{cde}) + \nabla^{(d}_{de} \varphi^{abc}] ]$ 

```

Do the actual chaining:

```

CollectTensors@MapTimedTensors[
  CollectTensors@SymmetrizeCovDs@CollectTensors[# /. rule2] &,
  O3ansatz
];
O123ansatz = CollectTensors[MapTimedTensors[
  CollectTensors@SymmetrizeCovDs@CollectTensors[# /. rule1] &,
  %
], Verbose -> True];

** Collecting tensors in expression of length 210 and head Plus.
** Expanded to 210 tensorial terms in 0.84s.
** Found 155 dummies, {a, b, c, d, e, 1$100781$107541, 1$100781$107627,
  1$100781$107694, 1$100781$107751, 1$100781$107828, <<145>>} in 1.46s.
** Replaced dummies in 2.26s.
** Applied TensorWrapper in 0.51s.
** Found 395 TensorWrappers in 0.02s.
** Canonicalized 395 TensorWrappers in 5.77s.
** Replaced TensorWrappers in 0.17s.
** Collected TensorWrappers in 1.27s.
** Simplified coefficient of each term in 0.32s.

```



```

O123ansatz = O123ansatz // ProjectRiemanns;

O123ansatz // Length
O123ansatz // TermsOf
O123ansatz // ConstantSymbolsOf

428

{ T ∇ ∇ R[∇] ∇ ∇ φ, T ∇ R[∇] ∇ ∇ ∇ φ, T ∇ φ ∇ ∇ ∇ R[∇],
  R[∇] T ∇ ∇ ∇ ∇ φ, T φ ∇ ∇ ∇ ∇ R[∇], T ∇ ∇ ∇ ∇ ∇ φ }

{ α1, α2, α3, α4, α5, α6, β1, β2, β3, β4, β5, β6, γ1, γ2, γ3, γ4, γ5, γ6 }

TensorPut [O123ansatz]

O123ansatz.m

TensorGet [O123ansatz]

O123ansatz.m

```

## 6.2 Non-factorization

In this section we try to demand that the gauge-invariant equations of motion are equal to the factorized equations of motion. This will turn out to be impossible.

```

TensorGet [eom]

eom.m

```

Restrict to the traceless part of the equations of motion. Since the traces of the equations of motion have to cancel by themselves, this is ok.

```

O123ansatzTF = O123ansatz /. T3 → T3TF;

```

Compare overall coefficients of terms without the Riemann tensor. The box cubed terms have the same coefficient, namely 1:

```

O123ansatzTF /. RiemannCD[___] → 0

```

$$\begin{aligned}
& \left( \frac{2 \alpha_5 \beta_5 \gamma_5}{9} + \frac{4 \alpha_6 \beta_5 \gamma_5}{9} + \frac{2 \alpha_5 \beta_6 \gamma_5}{9} + \frac{4 \alpha_6 \beta_6 \gamma_5}{9} \right) \text{Ttf}^{abc} \left( \nabla_{(abcdef)} \varphi^{def} \right) + \\
& \left( \frac{2 \alpha_5 \beta_5}{3} + \frac{2 \alpha_6 \beta_5}{3} + \frac{2 \alpha_5 \gamma_5}{3} + \frac{2 \alpha_6 \gamma_5}{3} + \frac{2 \beta_5 \gamma_5}{3} + \frac{2 \alpha_5 \beta_5 \gamma_5}{3} + \right. \\
& \quad \left. \frac{4 \alpha_6 \beta_5 \gamma_5}{9} + \frac{2 \beta_6 \gamma_5}{3} + \frac{4 \alpha_5 \beta_6 \gamma_5}{9} + \frac{2 \alpha_6 \beta_6 \gamma_5}{9} \right) \text{Ttf}^{abc} \left( \nabla_{(bcde}{}^f{}_{f)} \varphi_a{}^{de} \right) + \\
& \left( \alpha_5 + \beta_5 + \frac{\alpha_5 \beta_5}{3} + \gamma_5 + \frac{\alpha_5 \gamma_5}{3} + \frac{\beta_5 \gamma_5}{3} + \frac{\alpha_5 \beta_5 \gamma_5}{9} \right) \text{Ttf}^{abc} \left( \nabla_{(cd}{}^e{}^f{}_{ef)} \varphi_{ab}{}^d \right) + \\
& \text{Ttf}^{abc} \left( \nabla_{d}{}^{(de}{}^f{}_{ef)} \varphi_{abc} \right)
\end{aligned}$$

```

totaleom /. RiemannCD[___] → 0

```

$$\begin{aligned}
& -\frac{2}{5} \text{Ttf}^{abc} \left( \nabla_{(abcdef)} \varphi^{def} \right) + \frac{12}{5} \text{Ttf}^{abc} \left( \nabla_{(bcde}{}^f{}_{f)} \varphi_a{}^{de} \right) - \\
& 3 \text{Ttf}^{abc} \left( \nabla_{(cd}{}^e{}^f{}_{ef)} \varphi_{ab}{}^d \right) + \text{Ttf}^{abc} \left( \nabla_{d}{}^{(de}{}^f{}_{ef)} \varphi_{abc} \right)
\end{aligned}$$

If the equations of motion factorize, this should be zero:

```

shouldbezero = CollectTensors[totaleom - O123ansatzTF];

```

```

shouldbezero // Length
shouldbezero // ConstantSymbolsOf
shouldbezero // TermsOf
288

{A1, A10, A11, A13, A14, A15, A16, A17, A18, A20, A26, A36, A4, A46, A50, B1, B2, B3, B4, B5, B6,
B7, C10, C100, C101, C102, C103, C104, C105, C106, C107, C108, C109, C11, C110, C111, C112,
C113, C114, C115, C119, C120, C122, C123, C124, C126, C127, C130, C131, C132, C133, C135,
C136, C137, C138, C14, C140, C141, C15, C154, C155, C156, C157, C158, C16, C162, C165, C170,
C172, C173, C174, C175, C176, C177, C178, C179, C18, C180, C182, C184, C186, C200, C201, C203,
C211, C212, C221, C222, C245, C31, C32, C35, C38, C39, D1, D11, D12, D13, D14, D15, D16, D18,
D2, D3, D4, D5, D6, D7, α1, α2, α3, α4, α5, α6, β1, β2, β3, β4, β5, β6, γ1, γ2, γ4, γ5}

{Ttf ∇ ∇ R[∇] ∇ ∇ φ, Ttf ∇ R[∇] ∇ ∇ ∇ φ, Ttf ∇ φ ∇ ∇ ∇ R[∇],
R[∇] Ttf ∇ ∇ ∇ ∇ φ, Ttf φ ∇ ∇ ∇ ∇ R[∇], Ttf ∇ ∇ ∇ ∇ ∇ φ}

```

But there turns out to be an obstruction in terms that have a single derivative on Weyl tensors.

```

obstructionterms = Select[
  shouldbezero /. RiemannCD[____, a_, ___, b_, ____] /; PairQ[a, b] → 0 /.
  CD[a_] @ RiemannCD[____, b_, ____] /; PairQ[a, b] → 0,
  ! FreeQ[#, CD[_] @ RiemannCD[____]] &
];

```

```
List @@ obstructionterms // RemoveConstants
```

```

{ Ttfabc (∇g R[∇]adef) (∇(bcf) φdeg),
  Ttfabc (∇g R[∇]adef) (∇(cdf) φbeg), Ttfabc (∇a R[∇]defg) (∇(ceg) φbdf),
  Ttfabc (∇f R[∇]ad e) (∇(ceg) φdfg), Ttfabc (∇g R[∇]adef) (∇(cfg) φbde),
  Ttfabc (∇b R[∇]adef) (∇(cfg) φdeg), Ttfabc (∇f R[∇]ad e) (∇(cfg) φdeg),
  Ttfabc (∇f R[∇]ad e) (∇(c g) φdef), Ttfabc (∇f R[∇]ad e) (∇(deg) φcfg),
  Ttfabc (∇g R[∇]adef) (∇(dfg) φbce), Ttfabc (∇b R[∇]adef) (∇(dfg) φceg),
  Ttfabc (∇f R[∇]ad e) (∇(efg) φcdg), Ttfabc (∇c R[∇]ad e) (∇(efg) φdfg),
  Ttfabc (∇f R[∇]ad e) (∇(e g) φcdf), Ttfabc (∇b R[∇]adef) (∇(f g) φcde),
  Ttfabc (∇f R[∇]ad e) (∇(f g) φcde), Ttfabc (∇c R[∇]ad e) (∇(f g) φdef) }

```

```
SolveConstants[obstructionterms == 0]
```

```
{}
```

As tuning of the free coefficients is not sufficient to remove this obstruction (because the above SolveConstants doesn't give a solution), we can conclude that the obstruction to factorization is the first derivative of the Weyl tensor.

## 7 Weyl invariance

### 7.0 Description

In this section we show that the action is also invariant under the Weyl transformations

$$\begin{aligned}
 \varphi_{abc} &\rightarrow e^{4\Omega} \varphi_{abc}, \\
 g_{ab} &\rightarrow e^{2\Omega} g_{ab}.
 \end{aligned} \tag{5}$$

### 7.1 Branson's theorem: infinitesimal Weyl transformations

According to Branson (Math. Scand. 57 (1985), 293-345) invariance (or covariance) under infinitesimal Weyl transformations is sufficient for invariance (or covariance) under finite Weyl transformations. So instead of doing the full Weyl rescalings

$$\begin{aligned}\varphi_{abc} &\rightarrow e^{4\Omega} \varphi_{abc}, \\ g_{ab} &\rightarrow e^{2\Omega} g_{ab}.\end{aligned}\tag{6}$$

we can instead perform the perturbations

$$\begin{aligned}\delta_\Omega \varphi_{abc} &= 4\epsilon \Omega \varphi_{abc}, \\ \delta_\Omega g_{ab} &= 2\epsilon \Omega g_{ab},\end{aligned}\tag{7}$$

and demand that the action is invariant under them.

## 7.2 Check of Branson's theorem

In the section we perform a check on Branson's theorem; we derive that the only Weyl invariant 4-derivative action is the Weyl action.

**SetCurvatureRelations[CD]**

Rules {17, 18} have been declared as DownValues for RicciCD.

Rules {1, 2, 3, 4, 5, 6, 7, 8, 9, 10, <<6>>}  
have been declared as UpValues for RicciCD.

Rules {1, 2, 3, 4, 5, 6, 7, 8, 9, 10, <<4>>}  
have been declared as DownValues for RiemannCD.

Rules {1, 2, 3, 4, 5, 6, 7, 8, 9, 10, <<14>>}  
have been declared as DownValues for SymRiemannCD.

**ClearLinearRiemann[]**

**SetOptions[SymmetrizeCovDs, "UseCache" → False]**

{UseCache → False}

Check for invariance:

**ansatz = InvarLagrangian[metric, {4}]**

$$C_{n2}^{o2} R[\nabla]_{ab} R[\nabla]^{ab} + C_{n1}^{o2} R[\nabla]^2 + C_{n3}^{o2} R[\nabla]_{abcd} R[\nabla]^{abcd} + C_{n4}^{o2} (\nabla_a \nabla^a R[\nabla])$$

The last term is just a total derivative, so we have

**ansatz = Most@ansatz**

$$C_{n2}^{o2} R[\nabla]_{ab} R[\nabla]^{ab} + C_{n1}^{o2} R[\nabla]^2 + C_{n3}^{o2} R[\nabla]_{abcd} R[\nabla]^{abcd}$$

**eomTrace = metric[-a, -b] VarL[metric[-a, -b], CD][ansatz] //**  
**FullSimplification[] // CollectTensors**

$$(-6 C_{n1}^{o2} - 2 C_{n2}^{o2} - 2 C_{n3}^{o2}) (\nabla_a \nabla^a R[\nabla])$$

**SolveConstants[% == 0]**

Solve::svars : Equations may not give solutions for all "solve" variables. >>

$$\{ \{ C_{n3}^{o2} \rightarrow -3 C_{n1}^{o2} - C_{n2}^{o2} \} \}$$

**ansatz /. % // RiemannToWeyl // CollectTensors**

$$\left\{ \left( -6 C_{n1}^{o2} - C_{n2}^{o2} \right) R[\nabla]_{ab} R[\nabla]^{ab} + \left( 2 C_{n1}^{o2} + \frac{C_{n2}^{o2}}{3} \right) R[\nabla]^2 + \left( -3 C_{n1}^{o2} - C_{n2}^{o2} \right) W[\nabla]_{abcd} W[\nabla]^{abcd} \right\}$$

Up to total derivatives this is just Weyl squared, in accord with Branson's theorem:

```
% + (3 Cn1o2 + 1 / 2 Cn2o2) EulerDensity[CD] // RiemannToWeyl // CollectTensors
```

$$\left\{ \left( -6 C_{n1}^{o2} - \frac{3 C_{n2}^{o2}}{2} \right) W[\nabla]_{abcd} W[\nabla]^{abcd} \right\}$$

```
SetLinearRiemann[]
```

```
SetOptions[SymmetrizeCovDs, "UseCache" → True]
```

```
{UseCache → True}
```

```
ClearCurvatureRelations[CD]
```

Rules {17, 18} have been removed as DownValues for RicciCD.

Rules {1, 2, 3, 4, 5, 6, 7, 8, 9, 10, <<6>>} have been removed as UpValues for RicciCD.

Rules {1, 2, 3, 4, 5, 6, 7, 8, 9, 10, <<4>>}  
have been removed as DownValues for RiemannCD.

Rules {1, 2, 3, 4, 5, 6, 7, 8, 9, 10, <<14>>}  
have been removed as DownValues for SymRiemannCD.

### 7.3 Weyl invariance condition

We demand invariance of the action under infinitesimal Weyl transformations:

$$\begin{aligned} 0 &= \delta_\Omega S = \frac{\delta S}{\delta g_{ab}} \delta_\Omega g_{ab} + \frac{\delta S}{\delta \varphi_{abc}} \delta_\Omega \varphi_{abc} \\ &= \\ &\sqrt{-g} (\delta_\Omega g_{ab}) B^{ab} + \sqrt{-g} (\delta_\Omega \varphi_{abc}) O^{abcdef} \varphi_{def} + \frac{1}{2} \frac{\delta(\sqrt{-g} \varphi_{abc} O^{abcdef} \varphi_{def})}{\delta g_{gh}} \delta_\Omega g_{gh} \\ &= \sqrt{-g} 4 \Omega \varphi_{abc} O^{abcdef} \varphi_{def} + \frac{\delta(\sqrt{-g} \varphi_{abc} O^{abcdef} \varphi_{def})}{\delta g_{gh}} \Omega g_{gh}, \end{aligned} \quad (8)$$

leading to the single condition

$$\frac{1}{\sqrt{-g}} \frac{\delta(\sqrt{-g} \varphi_{abc} O^{abcdef} \varphi_{def})}{\delta g_{gh}} g_{gh} = -4 \varphi_{abc} O^{abcdef} \varphi_{def}. \quad (9)$$

It is possible to expand out the variation of the metric determinant on the LHS, but then we have to be careful with total derivatives. If we leave the metric determinant inside the variation, we can rewrite  $\varphi_{abc} O^{abcdef} \varphi_{def}$  on the LHS by adding total derivatives without it affecting the result.

We can only solve the zeroth order in Riemann tensors. This is because the perturbation of the Riemann tensor reads  $\delta R = \nabla \nabla \delta g$ :

```
RiemannCD[-a, -b, -c, d] // Perturbation // ExpandPerturbation
```

$$\begin{aligned} &\frac{1}{2} \left( -(\nabla_a \nabla_b \Delta g^{1d}_c) - \nabla_a \nabla_c \Delta g^{1d}_b + \nabla_a \nabla^d \Delta g^{1c}_b \right) + \\ &\frac{1}{2} \left( \nabla_b \nabla_a \Delta g^{1d}_c + \nabla_b \nabla_c \Delta g^{1d}_a - \nabla_b \nabla^d \Delta g^{1c}_a \right) \end{aligned}$$

so we need at least the  $(n+1)^{\text{th}}$  order in Riemanns in the equations of motion if we want to impose Weyl invariance to the  $n^{\text{th}}$  order in Riemanns.

This implies that the relevant part of a perturbation of a symmetrized covariant derivative of the Riemann tensor is just the symmetrized derivative of the perturbation of the Riemann tensor:  $\delta_\Omega \nabla_{(\dots)} R = \nabla_{(\dots)} (\delta_\Omega R)$ , irrespectively of any contractions in the derivatives.

## 7.4 Action rewritten with total derivatives

In this section we rewrite the action such that the part without Riemann tensors has 2 times 3 derivatives, instead of 6 derivatives. We do this because computing the variation of  $\varphi \nabla^6 \varphi$  with respect to the metric is very hard; that of  $\nabla^3 \varphi \nabla^3 \varphi$  is significantly easier.

The Ansatz for the action integrated by parts is:

```
actionPIansatz = MakeContractionAnsatz [
  IndexFree@{
    (* No curvature tensors. *)
    CD@CD@CD@phi CD@CD@CD@phi,
    (* One curvature tensor. *)
    phi RiemannCD CD@CD@CD@CD@phi,
    phi CD@RiemannCD CD@CD@CD@phi,
    phi CD@CD@RiemannCD CD@CD@phi,
    phi CD@CD@CD@RiemannCD CD@phi,
    phi CD@CD@CD@CD@RiemannCD phi
  },
  ConstantPrefix -> "p",
  Verbose -> True
];
```

Its equations of motion are:

```
actionPIeomansatz = ProjectRiemanns@CollectTensors@MapTimed [
  CollectTensors@SymmetrizeCovDs@
    CollectTensors[T3TF[-a, -b, -c] VarD[phi[-a, -b, -c], CD][#]] &,
  actionPIansatz
];
```

We demand that these equations of motion are equal to the ones we computed before:

```
SolveConstants [
  actionPIeomansatz == ProjectRiemanns[eom],
  ConstantSymbolsOf[actionPIeomansatz]
];
% // Dimensions
pisol = %[[1]];
```

Solve::svars : Equations may not give solutions for all "solve" variables. >>

```
{1, 91}
```

There is one solution, but still with a lot of unfixed coefficients of actionPIansatz. We set these to zero with the following rule:

```

nopsRule = # → 0 & /@Complement[
  ConstantSymbolsOf[actionPIansatz /. pisol],
  ConstantSymbolsOf[eom]
]

{p1 → 0, p10 → 0, p100 → 0, p101 → 0, p102 → 0, p103 → 0, p104 → 0, p105 → 0, p106 → 0, p107 → 0,
 p108 → 0, p109 → 0, p11 → 0, p110 → 0, p111 → 0, p112 → 0, p113 → 0, p114 → 0, p115 → 0,
 p116 → 0, p117 → 0, p118 → 0, p119 → 0, p12 → 0, p120 → 0, p121 → 0, p122 → 0, p123 → 0,
 p124 → 0, p125 → 0, p126 → 0, p127 → 0, p128 → 0, p129 → 0, p13 → 0, p130 → 0, p131 → 0,
 p132 → 0, p133 → 0, p134 → 0, p135 → 0, p136 → 0, p137 → 0, p138 → 0, p139 → 0, p14 → 0,
 p140 → 0, p141 → 0, p142 → 0, p143 → 0, p144 → 0, p145 → 0, p146 → 0, p147 → 0, p148 → 0,
 p149 → 0, p15 → 0, p150 → 0, p151 → 0, p152 → 0, p153 → 0, p154 → 0, p155 → 0, p156 → 0,
 p157 → 0, p158 → 0, p159 → 0, p16 → 0, p160 → 0, p161 → 0, p162 → 0, p163 → 0, p164 → 0,
 p165 → 0, p166 → 0, p167 → 0, p168 → 0, p169 → 0, p17 → 0, p170 → 0, p171 → 0, p172 → 0,
 p173 → 0, p174 → 0, p175 → 0, p176 → 0, p177 → 0, p178 → 0, p179 → 0, p18 → 0, p180 → 0,
 p181 → 0, p182 → 0, p183 → 0, p184 → 0, p185 → 0, p186 → 0, p187 → 0, p188 → 0, p189 → 0,
 p19 → 0, p190 → 0, p191 → 0, p192 → 0, p193 → 0, p194 → 0, p195 → 0, p196 → 0, p197 → 0,
 p198 → 0, p2 → 0, p20 → 0, p201 → 0, p202 → 0, p203 → 0, p205 → 0, p206 → 0, p207 → 0, p209 → 0,
 p21 → 0, p211 → 0, p212 → 0, p213 → 0, p214 → 0, p215 → 0, p216 → 0, p22 → 0, p221 → 0,
 p222 → 0, p223 → 0, p224 → 0, p225 → 0, p226 → 0, p227 → 0, p228 → 0, p229 → 0, p23 → 0,
 p230 → 0, p232 → 0, p233 → 0, p236 → 0, p237 → 0, p24 → 0, p241 → 0, p242 → 0, p243 → 0,
 p244 → 0, p245 → 0, p246 → 0, p247 → 0, p248 → 0, p249 → 0, p25 → 0, p250 → 0, p252 → 0,
 p253 → 0, p26 → 0, p261 → 0, p263 → 0, p264 → 0, p269 → 0, p27 → 0, p270 → 0, p271 → 0,
 p28 → 0, p282 → 0, p287 → 0, p289 → 0, p3 → 0, p31 → 0, p32 → 0, p33 → 0, p34 → 0, p35 → 0,
 p36 → 0, p37 → 0, p38 → 0, p39 → 0, p40 → 0, p41 → 0, p42 → 0, p43 → 0, p44 → 0, p45 → 0,
 p46 → 0, p47 → 0, p48 → 0, p49 → 0, p50 → 0, p51 → 0, p52 → 0, p53 → 0, p56 → 0, p57 → 0,
 p61 → 0, p62 → 0, p70 → 0, p71 → 0, p72 → 0, p73 → 0, p74 → 0, p77 → 0, p78 → 0, p79 → 0}

```

The final action integrated by parts is then:

```
actionPI = actionPIansatz /. pisol /. nopsRule;
```

```
TensorPut[actionPI]
```

```
actionPI.m
```

## 7.5 Trace of the energy-momentum tensor and invariance

In this subsection we compute the trace of the energy-momentum tensor, namely

$$T = \frac{1}{\sqrt{-g}} \frac{\delta(\sqrt{-g} \varphi_{abc} O^{abcdef} \varphi_{def})}{\delta g_{gh}} g_{gh}.$$

We only compute it up to zeroth order in Riemann tensors, after taking the variation w.r.t. the metric all derivatives commute and are symmetric. To impose this, we use the following function:

```

ToSymmetricDerivatives[expr_] :=
  CollectTensors[expr /. CD[a__]@CD[b__][x_] => CD[a, b][x]];

```

The first part of the trace of  $T_{ab}$  ("traceA") comes from the action without Riemann tensors:

```

traceA = CollectTensors@MapTimedTensors[
  ToSymmetricDerivatives[metric[-a, -b] VarL[metric[-a, -b], CD][#]] &,
  actionPI /. RiemannCD[___] → 0 // ExpandSymCovDs // CollectTensors
];

```

```
traceA // TermsOf
```

```
traceA // Length
```

```
{∇ ∇ ∇ ∇ φ2, ∇ ∇ φ ∇ ∇ ∇ ∇ φ, ∇ φ ∇ ∇ ∇ ∇ ∇ ∇ φ, φ ∇ ∇ ∇ ∇ ∇ ∇ φ}
```

The second part of the trace of  $T_{ab}$  ("traceB") comes from the part of the action with Riemann tensors. Because we compute to zeroth order in Riemanns, it suffices here to just replace the Riemann tensors with the perturbation w.r.t. the metric. We first make a rule for this:

```
RiemannCD[-a, -b, -c, d]
% // Perturbation // ExpandPerturbation // ToSymmetricDerivatives
δriemannRule = MakeRule@Evaluate@{%%, %}

R[∇]_{abc}^d

- 1/2 (∇_{(ac)} Δg^1_b^d) + 1/2 (∇_{(a}^d Δg^1_{bc}) + 1/2 (∇_{(bc)} Δg^1_a^d) - 1/2 (∇_{(b}^d Δg^1_{ac})

{HoldPattern[R[∇]_{abc}^d] :=
Module[{ }, - 1/2 (∇^{(ac)} Δg^{1bd}) + 1/2 (∇^{(ad)} Δg^{1bc}) + 1/2 (∇^{(bc)} Δg^{1ad}) - 1/2 (∇^{(bd)} Δg^{1ac}) ]}
```

We can now compute the actual contribution to the trace, "traceB":

```
traceB =
CollectTensors@MapTimedTensors[
ToSymmetricDerivatives[
metric[-a, -b] VarD[Perturbationmetric[LI[1], -a, -b], CD][
# /. δriemannRule // CollectTensors] /. delta[-LI[1], LI[1]] → 1] &,
Select[actionPI /. nops, ! FreeQ[#, RiemannCD] &]
];
```

The full trace to zeroth order in the Riemann tensor is then:

```
trace = traceA + traceB // CollectTensors

4/5 φ^{abc} (∇_{(abcdef)} φ^{def}) - 24/5 φ^{abc} (∇_{(bcde}^f φ_a^{de}) +
6 φ^{abc} (∇_{(cd}^e φ_{ef}) φ_{ab}^d) - 2 φ^{abc} (∇_{d}^{(de} φ_{ef}) φ_{abc})
```

This is precisely -4 times the zeroth order part of the action:

```
-4 action /. RiemannCD[___] → 0 // Expand

4/5 φ^{abc} (∇_{(abcdef)} φ^{def}) - 24/5 φ^{abc} (∇_{(bcde}^f φ_a^{de}) +
6 φ^{abc} (∇_{(cd}^e φ_{ef}) φ_{ab}^d) - 2 φ^{abc} (∇_{d}^{(de} φ_{ef}) φ_{abc})
```

Indeed, their difference is zero:

```
% - %%
0
```

So the condition

$$\frac{1}{\sqrt{-g}} \frac{\delta(\sqrt{-g} \varphi_{abc} O^{abcdef} \varphi_{def})}{\delta g_{gh}} g_{gh} = -4 \varphi_{abc} O^{abcdef} \varphi_{def}, \quad (10)$$

is satisfied, and we have proven that the action is invariant under Weyl transformations.
